# Supplementary material for: Type Ia supernovae with and without blueshifted narrow Na I D lines - how different is their structure?
Source: arXiv:1707.00700 ancillary file (2017-07-03)
Supplement: Supplementary file 1 [file suppA-NaId-SN-structanalysis.pdf]

# Supplementary material A: Type Ia supernovae with and without blueshifted narrow Na I D lines – how different is their structure?

S. Hachinger[1,2,3], F. K. Röpke[1,4], P. A. Mazzali[5,6], A. Gal-Yam[7], K. Maguire[8,9], M. Sullivan[10], S. Taubenberger[8,6], C. Ashall[5], H. Campbell[11], N. Elias-Rosa[12], U. Feindt[13], L. Greggio[12], C. Inserra[9], M. Miluzio[12,14], S. J. Smartt[9], D. Young[9]

[1]*Institut für Theoretische Physik und Astrophysik, Universität Würzburg, Emil-Fischer-Str. 31, 97074 Würzburg, Germany*
[2]*Institut für Mathematik, Universität Würzburg, Emil-Fischer-Str. 30, 97074 Würzburg, Germany*
[3]*Leibniz Supercomputing Centre (LRZ), Bavarian Academy of Sciences and Humanities, Boltzmannstr. 1, 85748 Garching b. München, Germany*
[4]*Heidelberger Institut für Theoretische Studien, Schloss-Wolfsbrunnenweg 35, 69118 Heidelberg, Germany*
[5]*Astrophysics Research Institute, Liverpool John Moores University, IC2 Liverpool Science Park, 146 Brownlow Hill, Liverpool, L3 5RF, UK*
[6]*Max-Planck-Institut für Astrophysik, Karl-Schwarzschild-Str. 1, 85741 Garching, Germany*
[7]*Benoziyo Center for Astrophysics, Weizmann Institute of Science, 76100 Rehovot, Israel*
[8]*European Organisation for Astronomical Research in the Southern Hemisphere (ESO), Karl-Schwarzschild-Str. 2, 85748 Garching b. München, Germany*
[9]*School of Mathematics and Physics, Queen's University Belfast, Belfast BT7 1NN, UK*
[10]*Physics & Astronomy, University of Southampton, Southampton, Hampshire SO17 1BJ, UK*
[11]*Institute of Astronomy, University of Cambridge, Madingley Road, Cambridge CB3 0HA, UK*
[12]*INAF - Osservatorio Astronomico di Padova, vicolo dell'Osservatorio 5, 35122 Padova, Italy*
[13]*Oskar Klein Centre, Department of Physics, Stockholm University, Albanova University Center, 10691 Stockholm, Sweden*
[14]*Instituto de Astrofisica de Canarias, C/ Vía Láctea, s/n, 38205, La Laguna, Tenerife, Spain*

**ABSTRACT**

This supplementary data appendix gives details on all our spectral models for Type Ia supernovae (SNe Ia) discussed and evaluated in the main paper (references see there). We have modelled the low-resolution spectra of 13 SNe Ia, obtaining photospheric velocities, model luminosities and abundance distributions, i.e. structural information on the SNe. Below, we first show an atlas of spectral fits (Section 1) and then an atlas of abundance distributions (Section 2) for our objects. Raw model input and output data can be obtained from the corresponding author S. Hachinger upon request by e-mail (hachinger@lrz.de).

## 1 ATLAS OF SPECTRAL FITS (WITH DATA ON LUMINOSITIES/PHOTOSPHERIC VELOCITIES)

Below we show our spectral fits based on the N100 density model (cf. main paper). Model luminosities and photospheric velocities can be read from the plots.

Some of our models – especially those for the SNe 2002ha (Figure 2), LSQ12fxd (Figure 1) and SNF20080514-002 (Figure 10) – show a somewhat worse fit quality than usual in detailed 'Abundance Tomography' modelling of SNe. With comparison to these studies on individual, extremely well-observed objects, we have modelled our objects with a reduced number of free fit parameters and less spectra per object on average (cf. main text). In addition, there has been a higher uncertainty in distance and/or reddening for some objects modelled (e.g. SNe 2002ha and LSQ12fxd). Thus, some mismatch from models to data is expected. The uncertainties generated by this in the final results (main text, Section 4) are expected to be within the error bars given and discussed in the main text.

© 2017 The Authors. Journal compilation © 2017 RAS

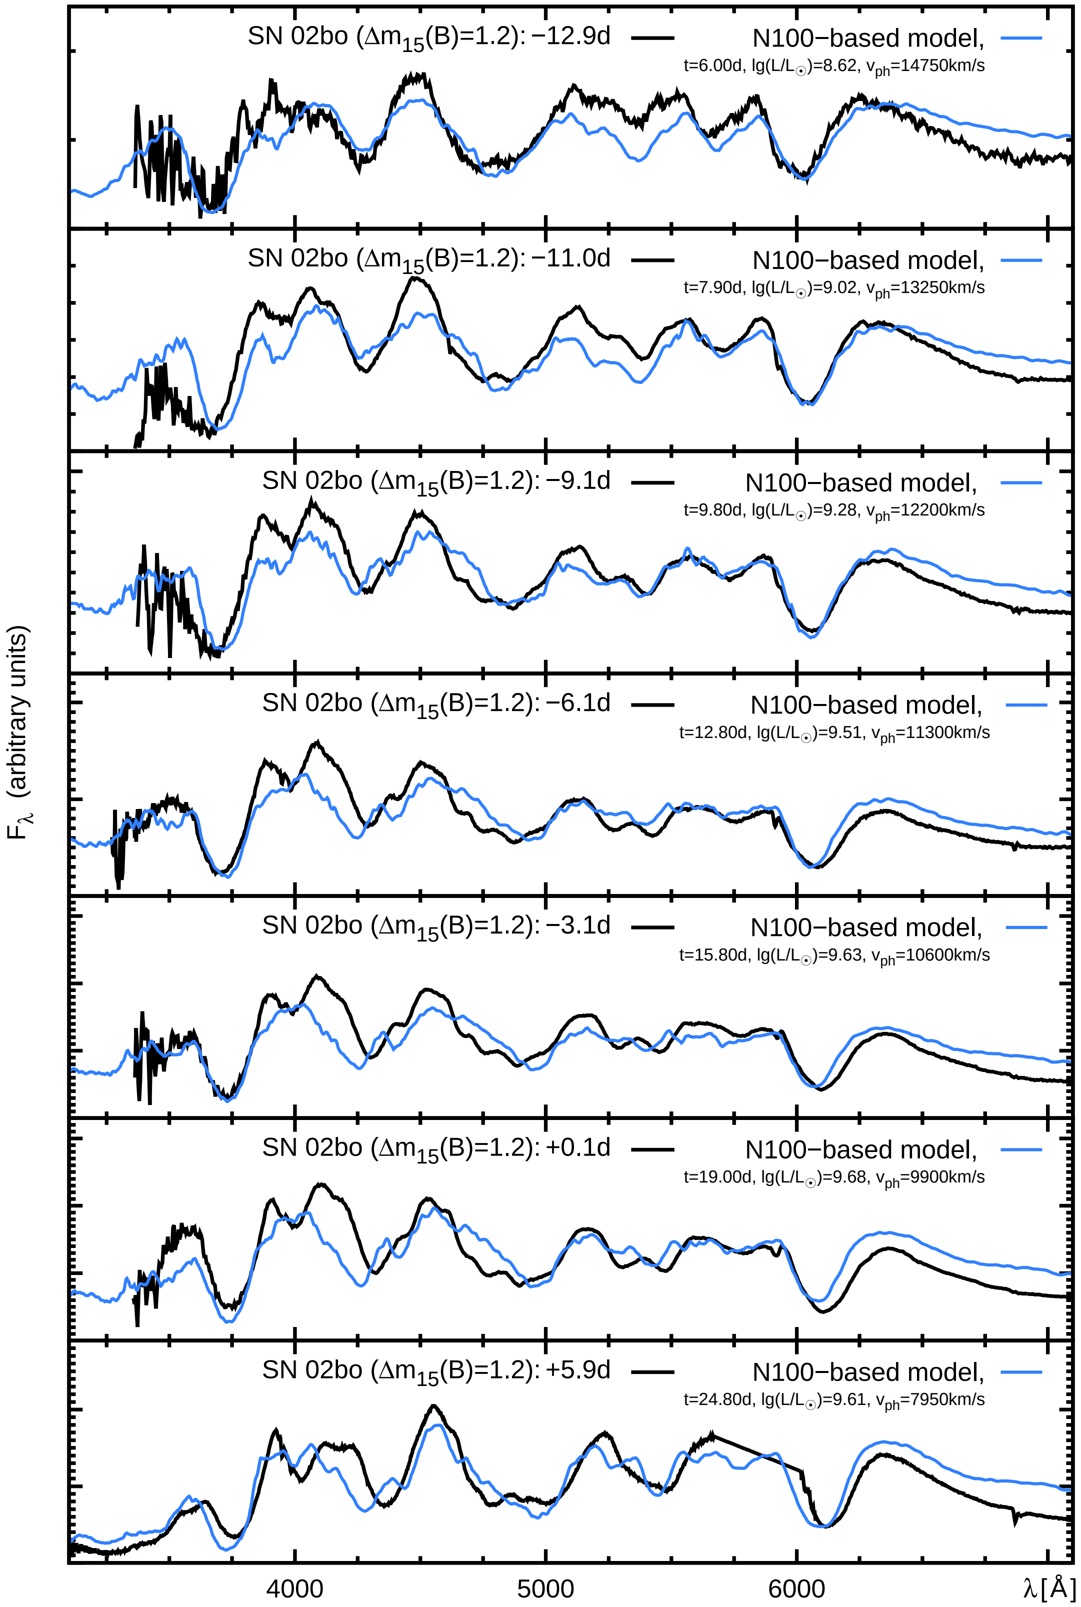


**Figure 1.** Model sequence for the 'blueshifted-Na' SN 2002bo (blue lines). The observed (low-resolution) spectra (black lines) are plotted for comparison.

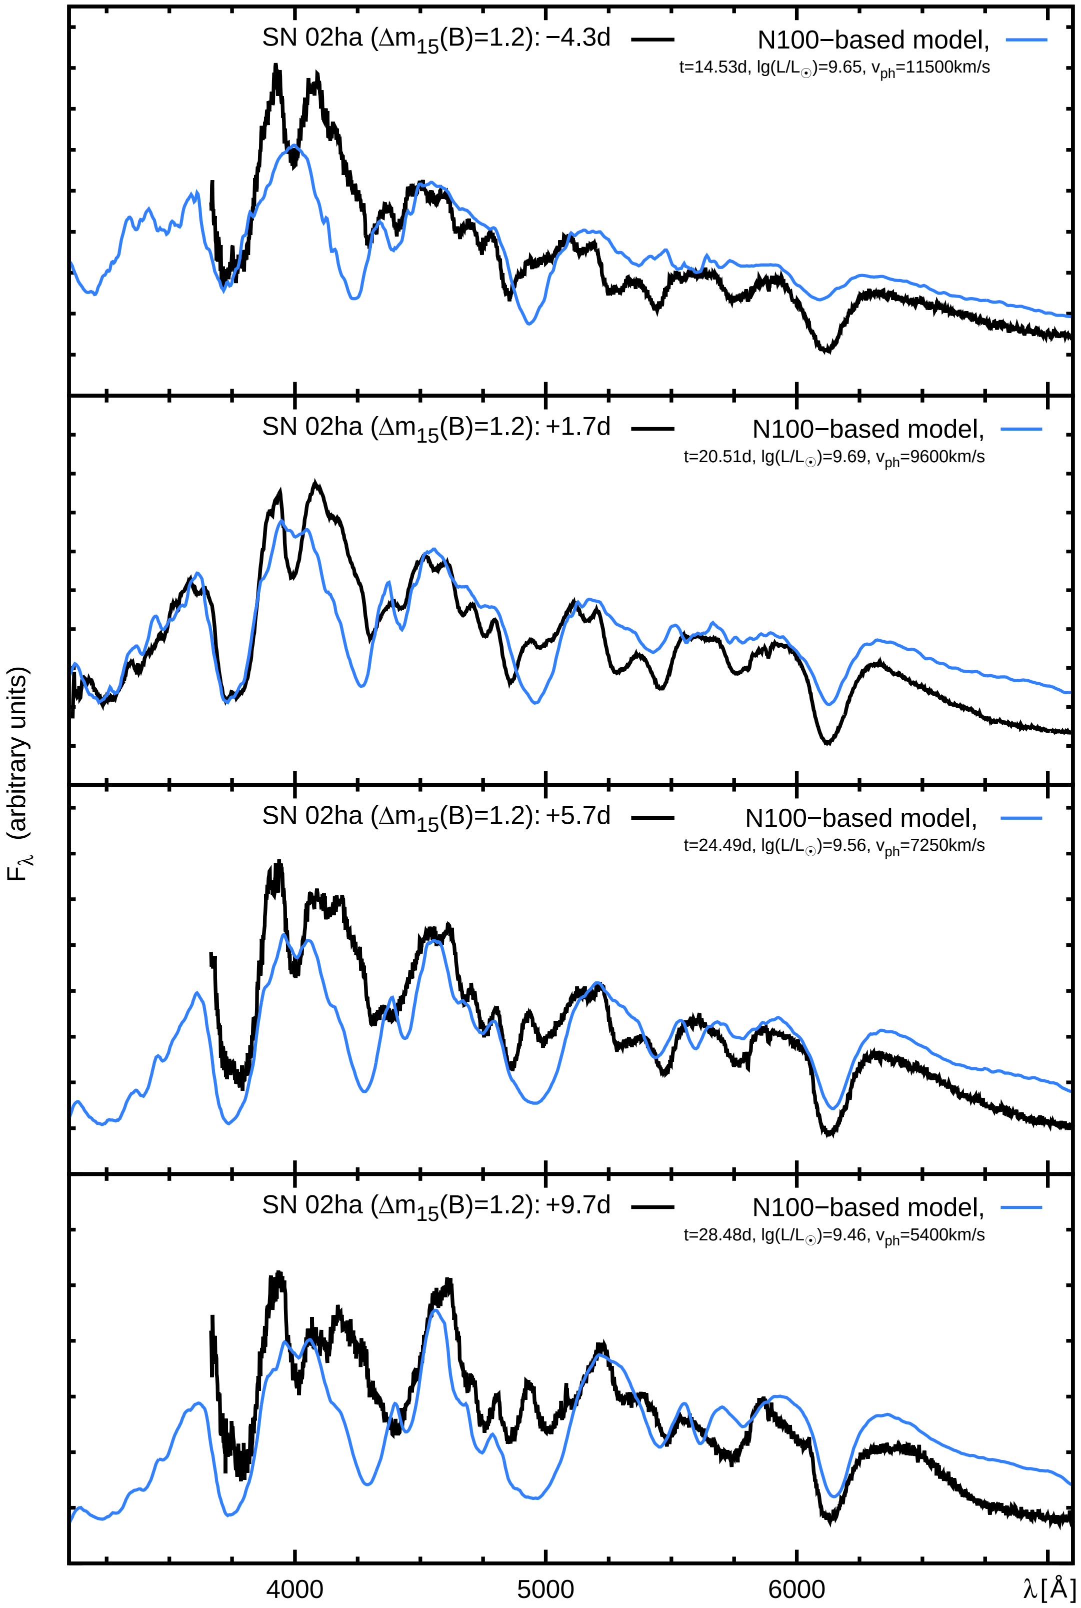


**Figure 2.** Model sequence for the 'blueshifted-Na' SN 2002ha (blue lines). The observed (low-resolution) spectra (black lines) are plotted for comparison. Plot analogous to Figure 1. The fit quality is worse than average as the model generally shows an ionisation degree somewhat too high (possibly owing to an underestimated distance or overestimated reddening, effectively-leading to an overestimated SN luminosity). The strong absorption at $\sim 4800$ Å in the model is due to Fe III lines; Si II lines ($\lambda$4130, $\lambda$5972, $\lambda$6355), favoured when the ionisation is lower, are reduced in turn. The abundance structure we derive for this object may be somewhat less reliable.

© 2017 The Authors. Journal compilation © 2017 RAS, MNRAS

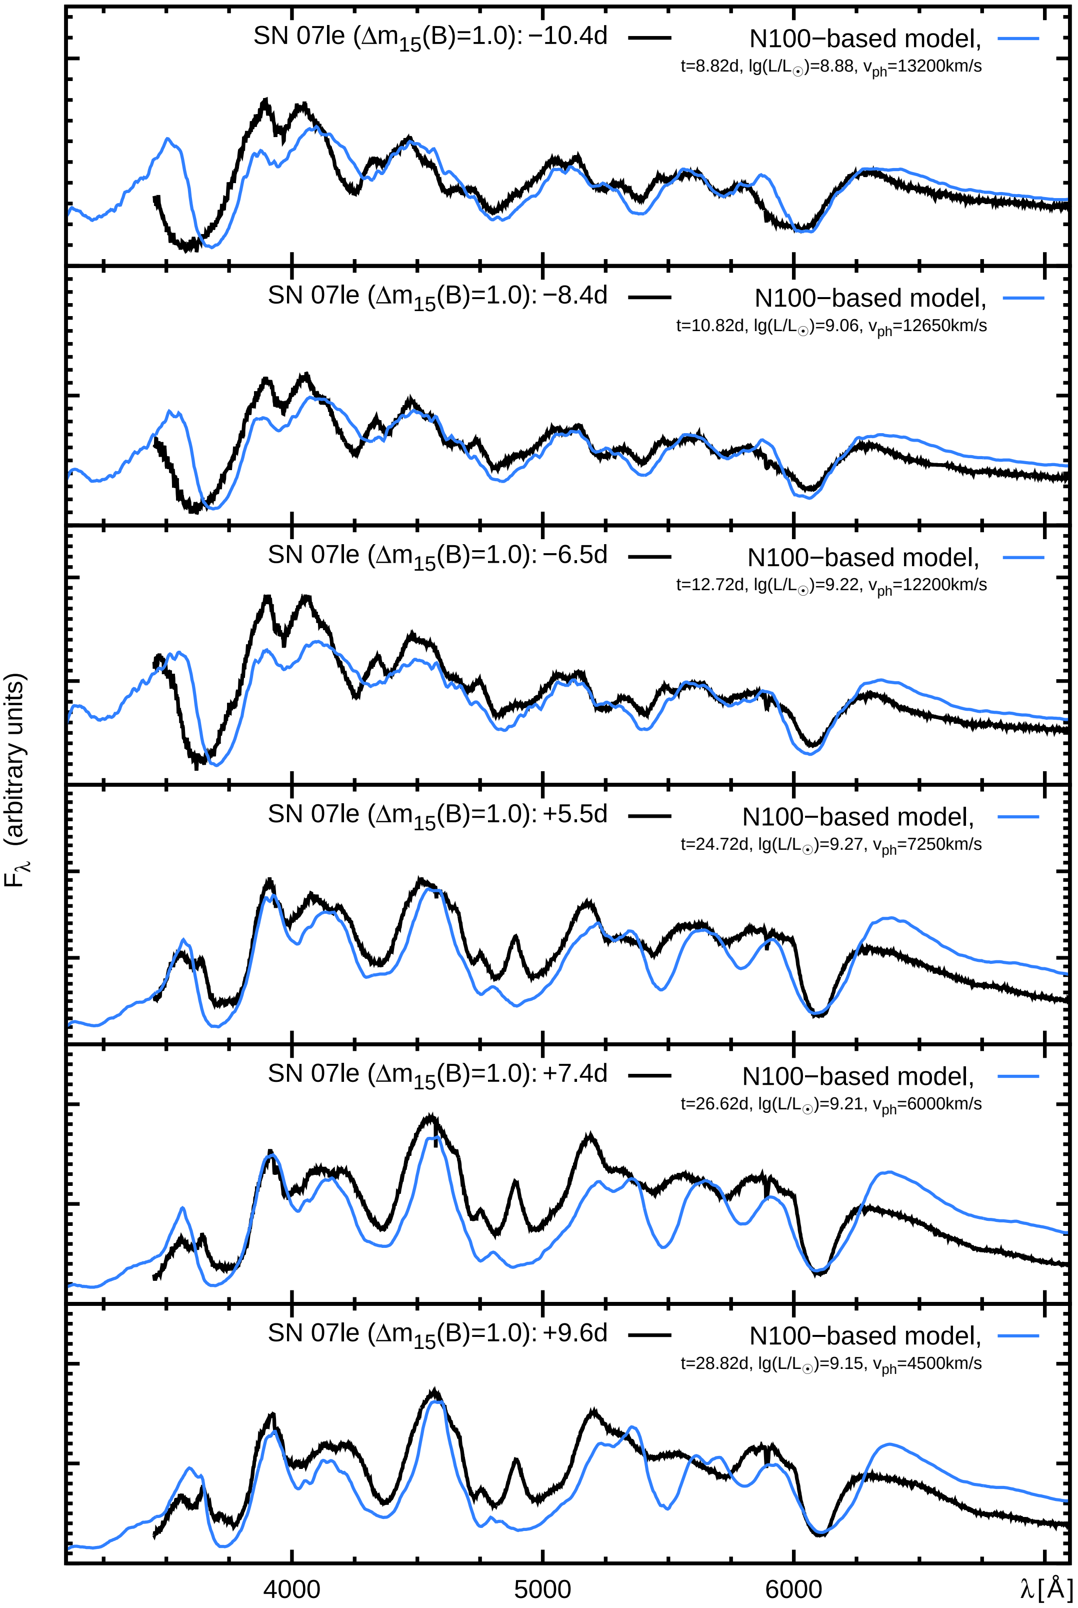


**Figure 3.** Model sequence for the 'blueshifted-Na' SN 2007le (blue lines). The observed (low-resolution) spectra (black lines) are plotted for comparison. Analogous to Figure 1.

© 2017 The Authors. Journal compilation © 2017 RAS, MNRAS

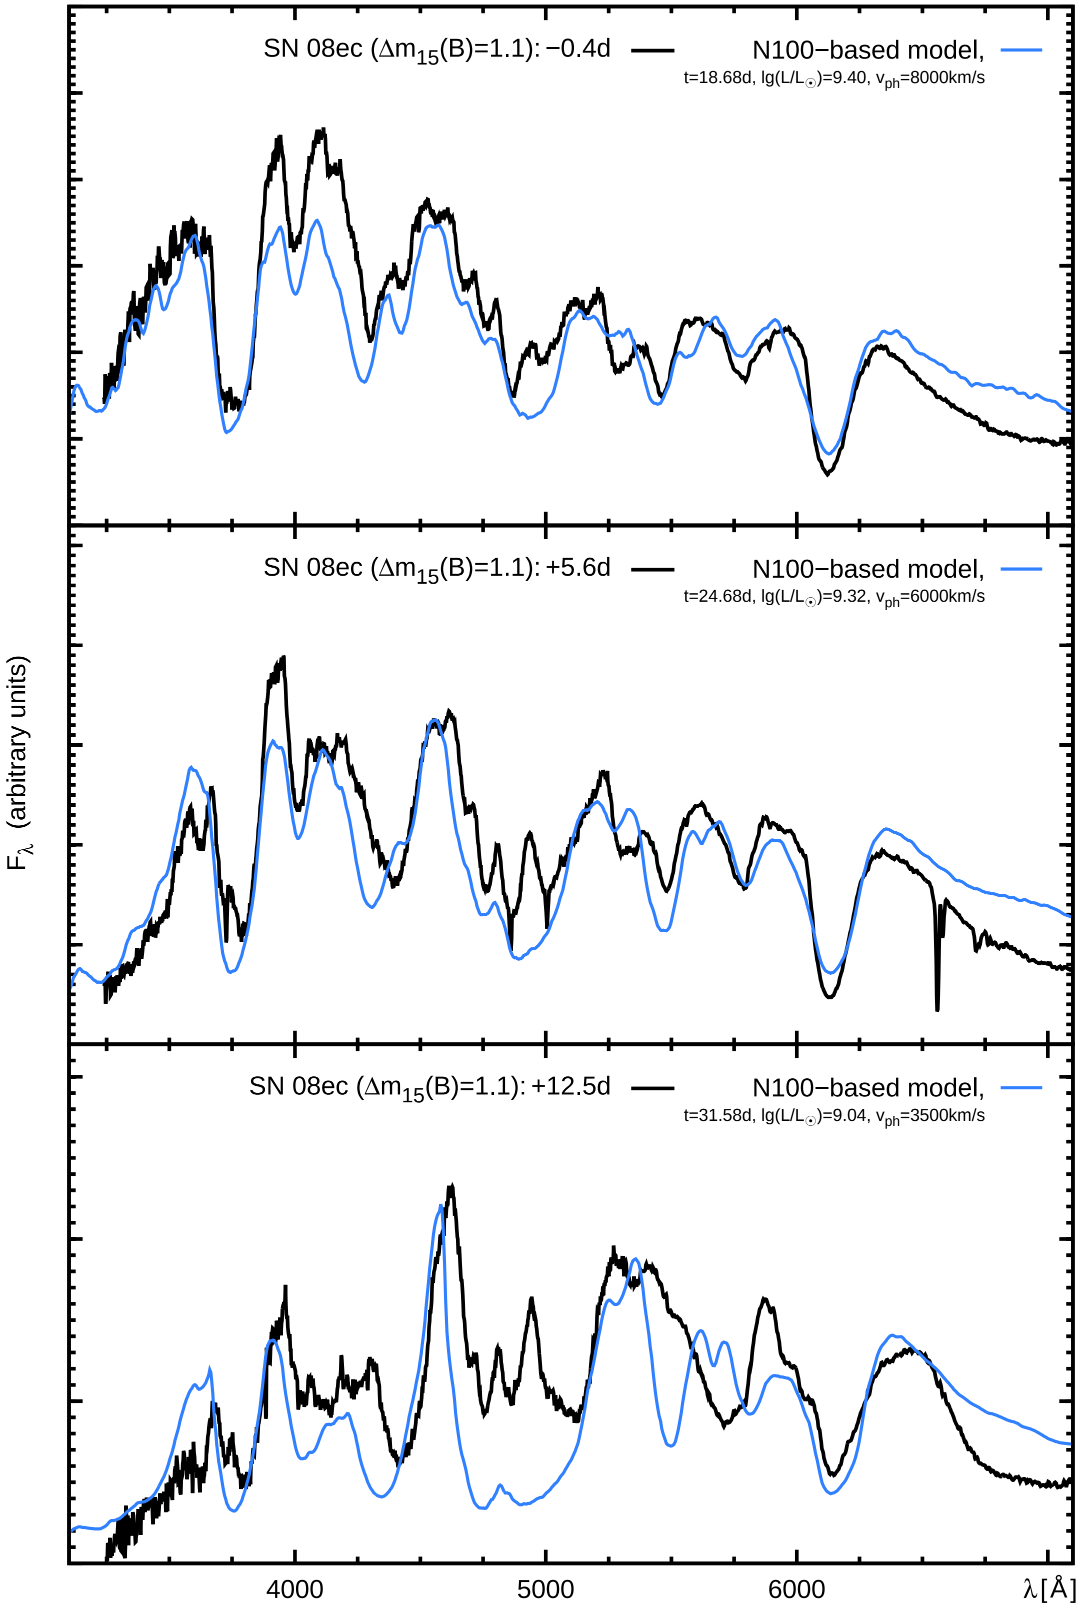


**Figure 4.** Model sequence for the 'blueshifted-Na' SN 2008ec (blue lines). The observed (low-resolution) spectra (black lines) are plotted for comparison. Analogous to Figure 1.

© 2017 The Authors. Journal compilation © 2017 RAS, MNRAS

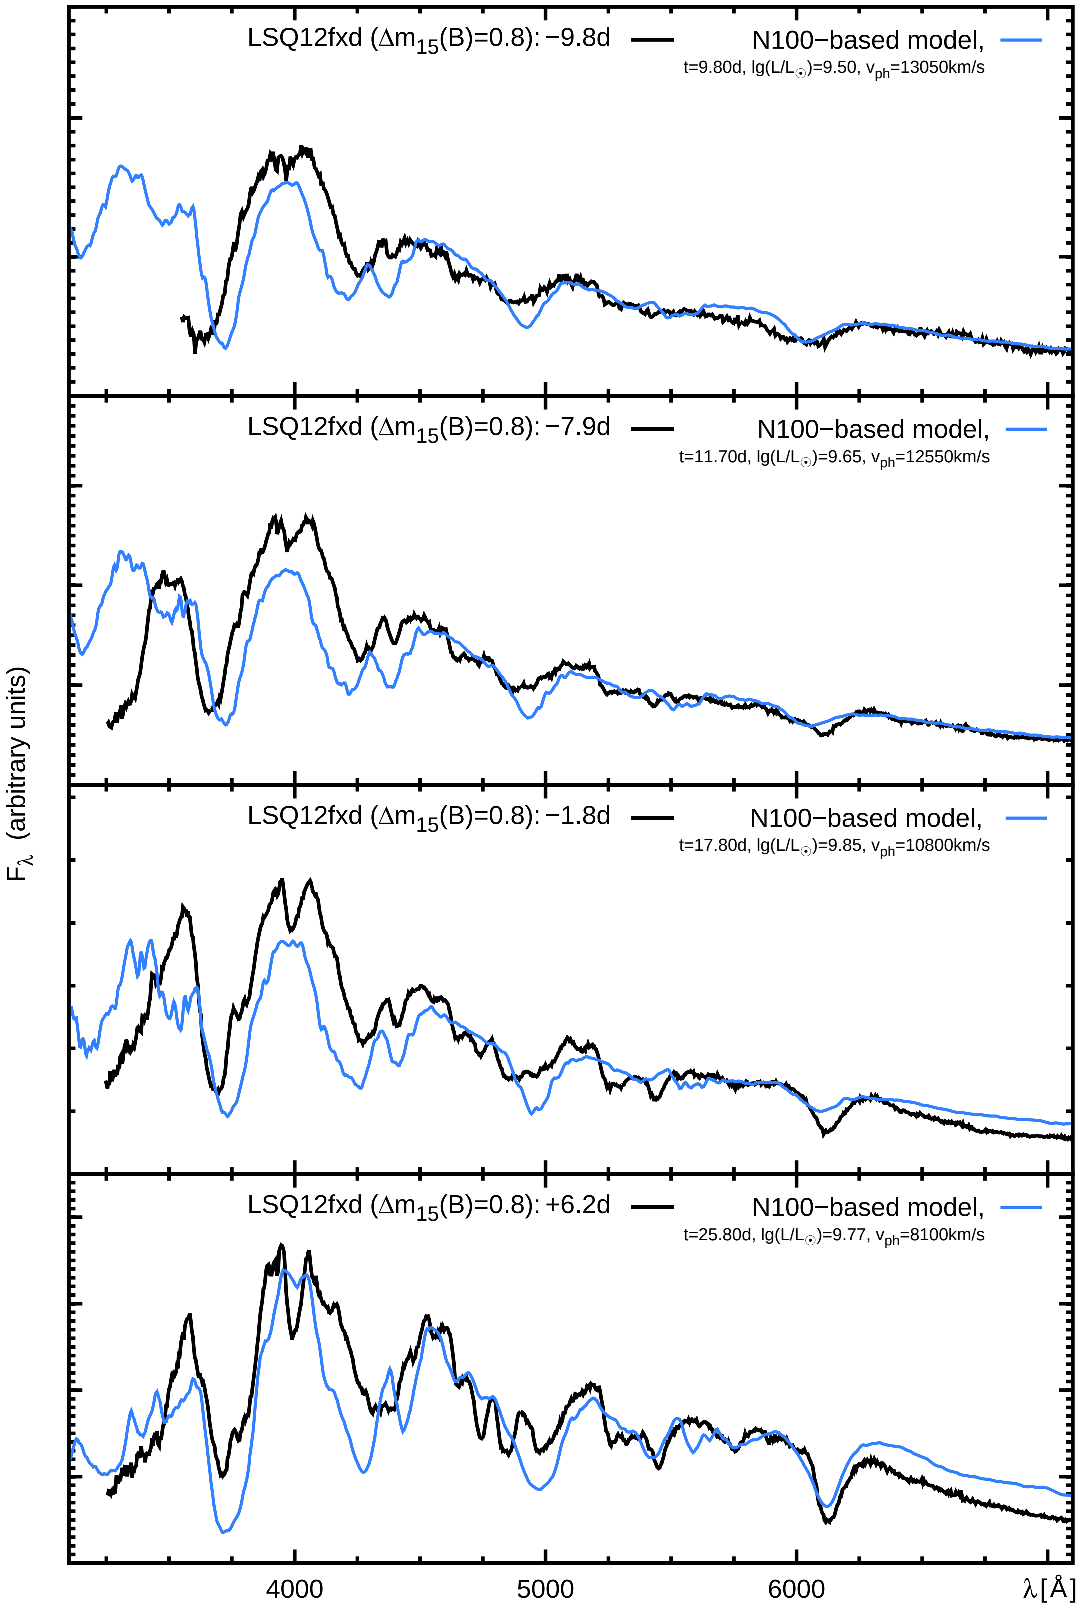


**Figure 5.** Model sequence for the 'blueshifted-Na' SN LSQ 12fxd (blue lines). The observed (low-resolution) spectra (black lines) are plotted for comparison. Analogous to Figure 1. For modelling LSQ 12fxd, we have assumed a redshift-based distance modulus of 35.58 ($H_0 = 72$km s$^{-1}$ Mpc$^{-1}$; reference frame 3K CMB) from NED as well as a lower-limit reddening of 0.08 (cf. main text); with the redshift-independent value from NED (35.98) and higher reddening values, the ionisation equilibrium within the ejecta model was too hot for reasonably matching the observations. Some mismatches in line strength remain (similar as in the fits to SN 2002ha, Figure 2).

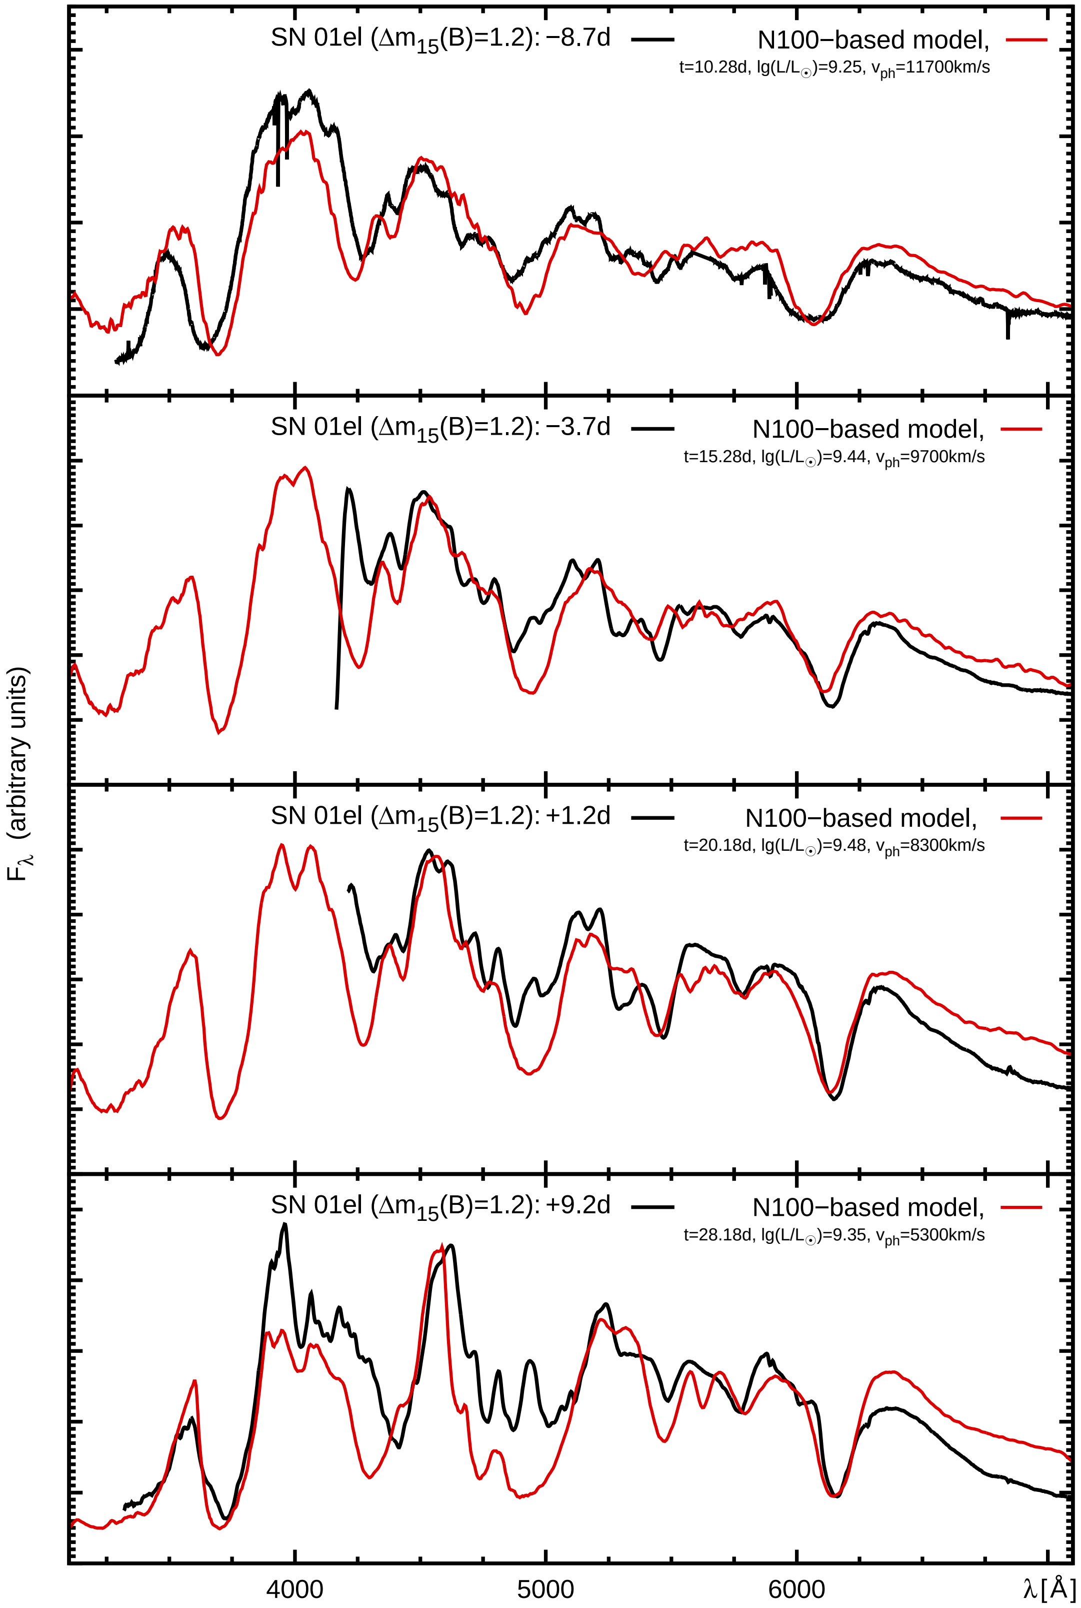


**Figure 6.** Model sequence for the 'redshifted-Na' SN 2001el (red lines). The observed (low-resolution) spectra (black lines) are plotted for comparison. Analogous to Figure 1.

© 2017 The Authors. Journal compilation © 2017 RAS, MNRAS

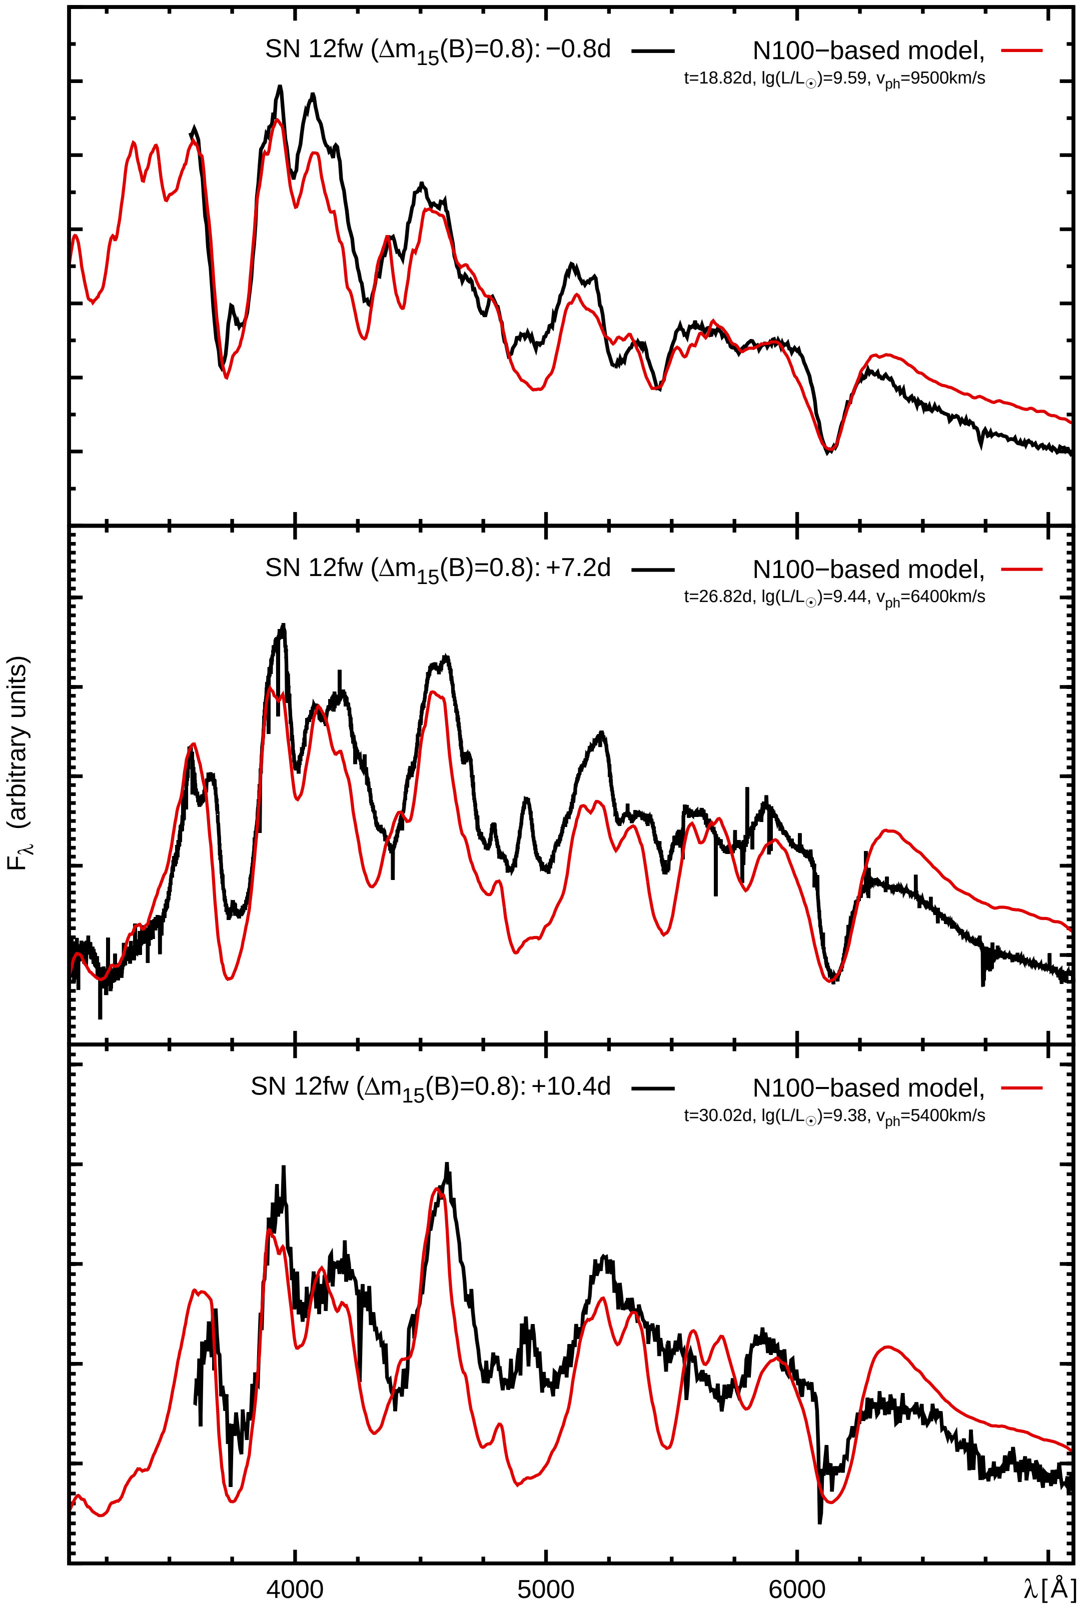


**Figure 7.** Model sequence for the 'redshifted-Na' SN 2012fw (red lines). The observed (low-resolution) spectra (black lines) are plotted for comparison. Analogous to Figure 1.

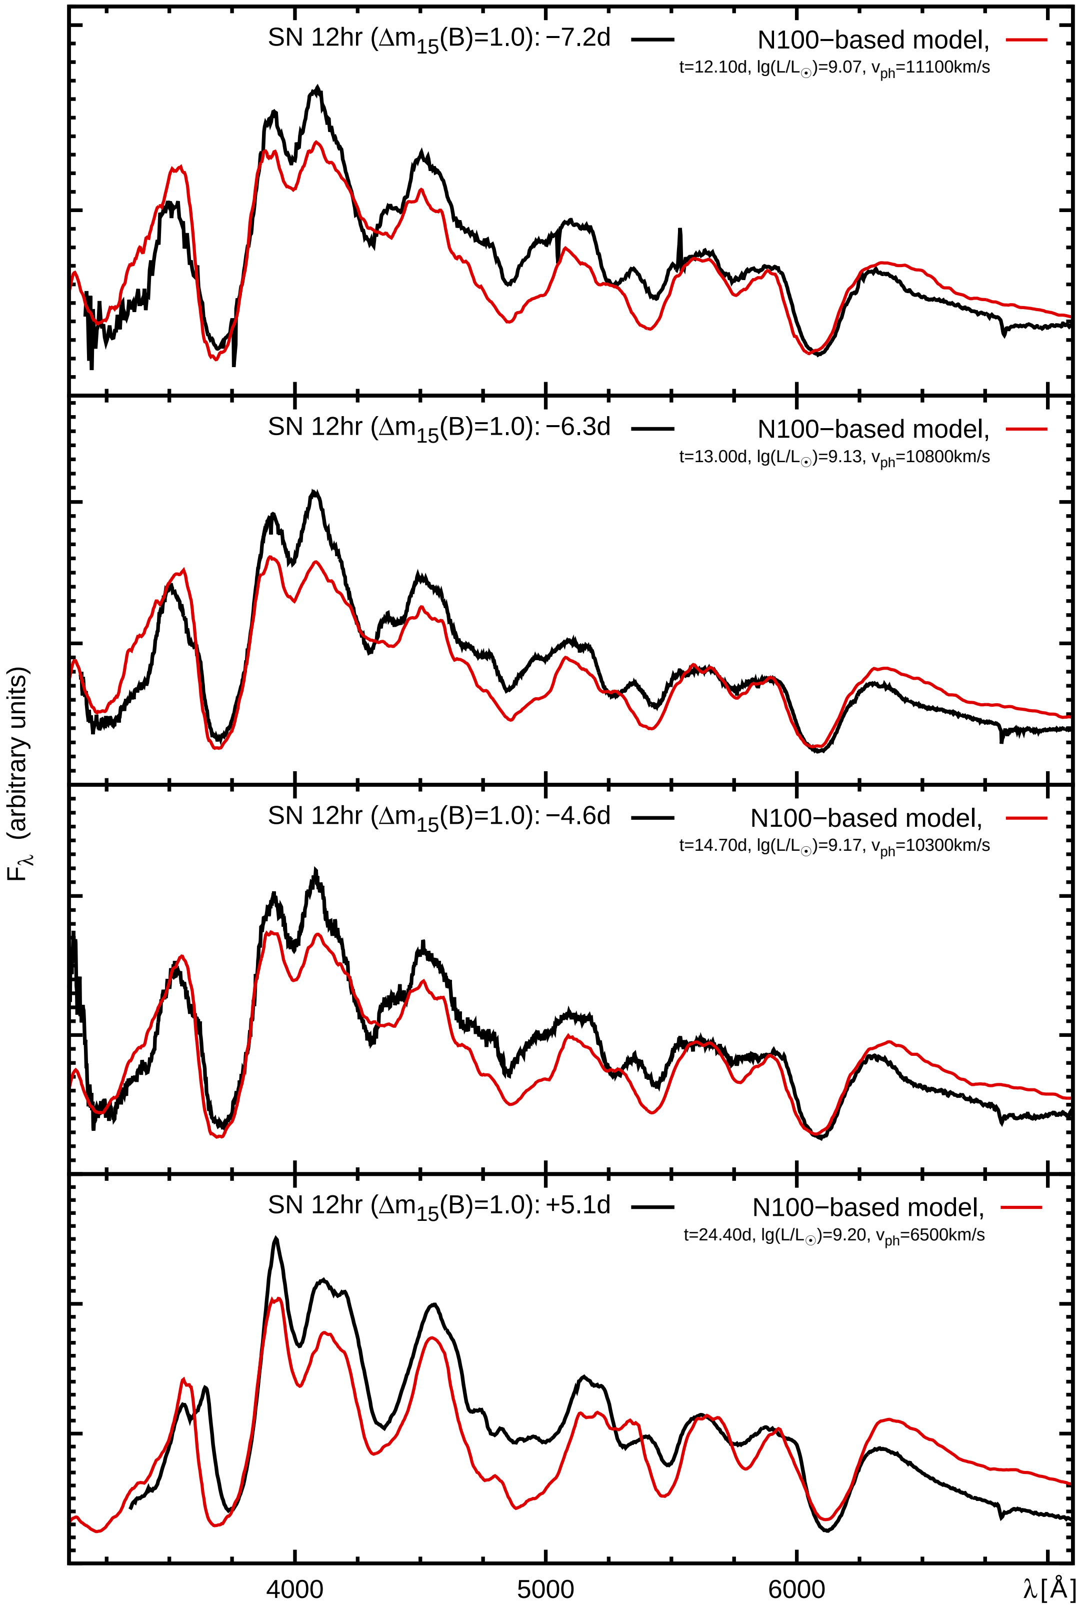


**Figure 8.** Model sequence for the 'redshifted-Na' SN 2012hr (red lines). The observed (low-resolution) spectra (black lines) are plotted for comparison. Analogous to Figure 1.

© 2017 The Authors. Journal compilation © 2017 RAS, MNRAS

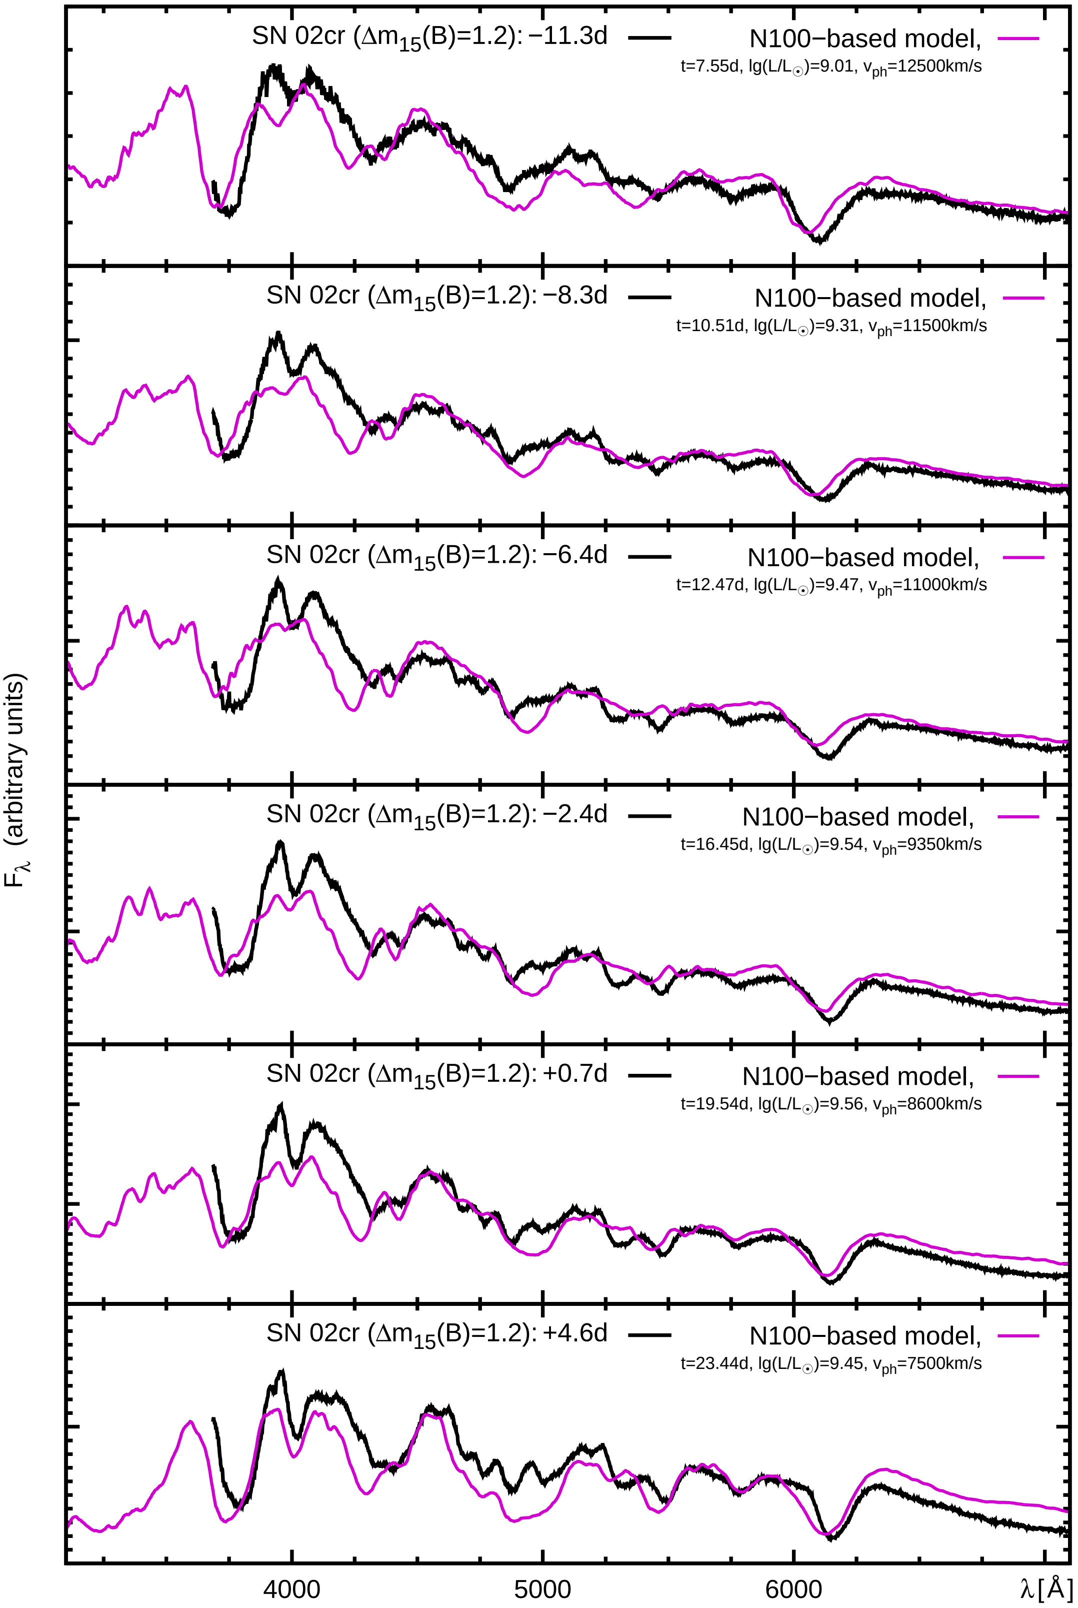


**Figure 9.** Model sequence for the 'single-Na' SN 2002cr (violet lines). The observed (low-resolution) spectra (black lines) are plotted for comparison. Analogous to Figure 1.

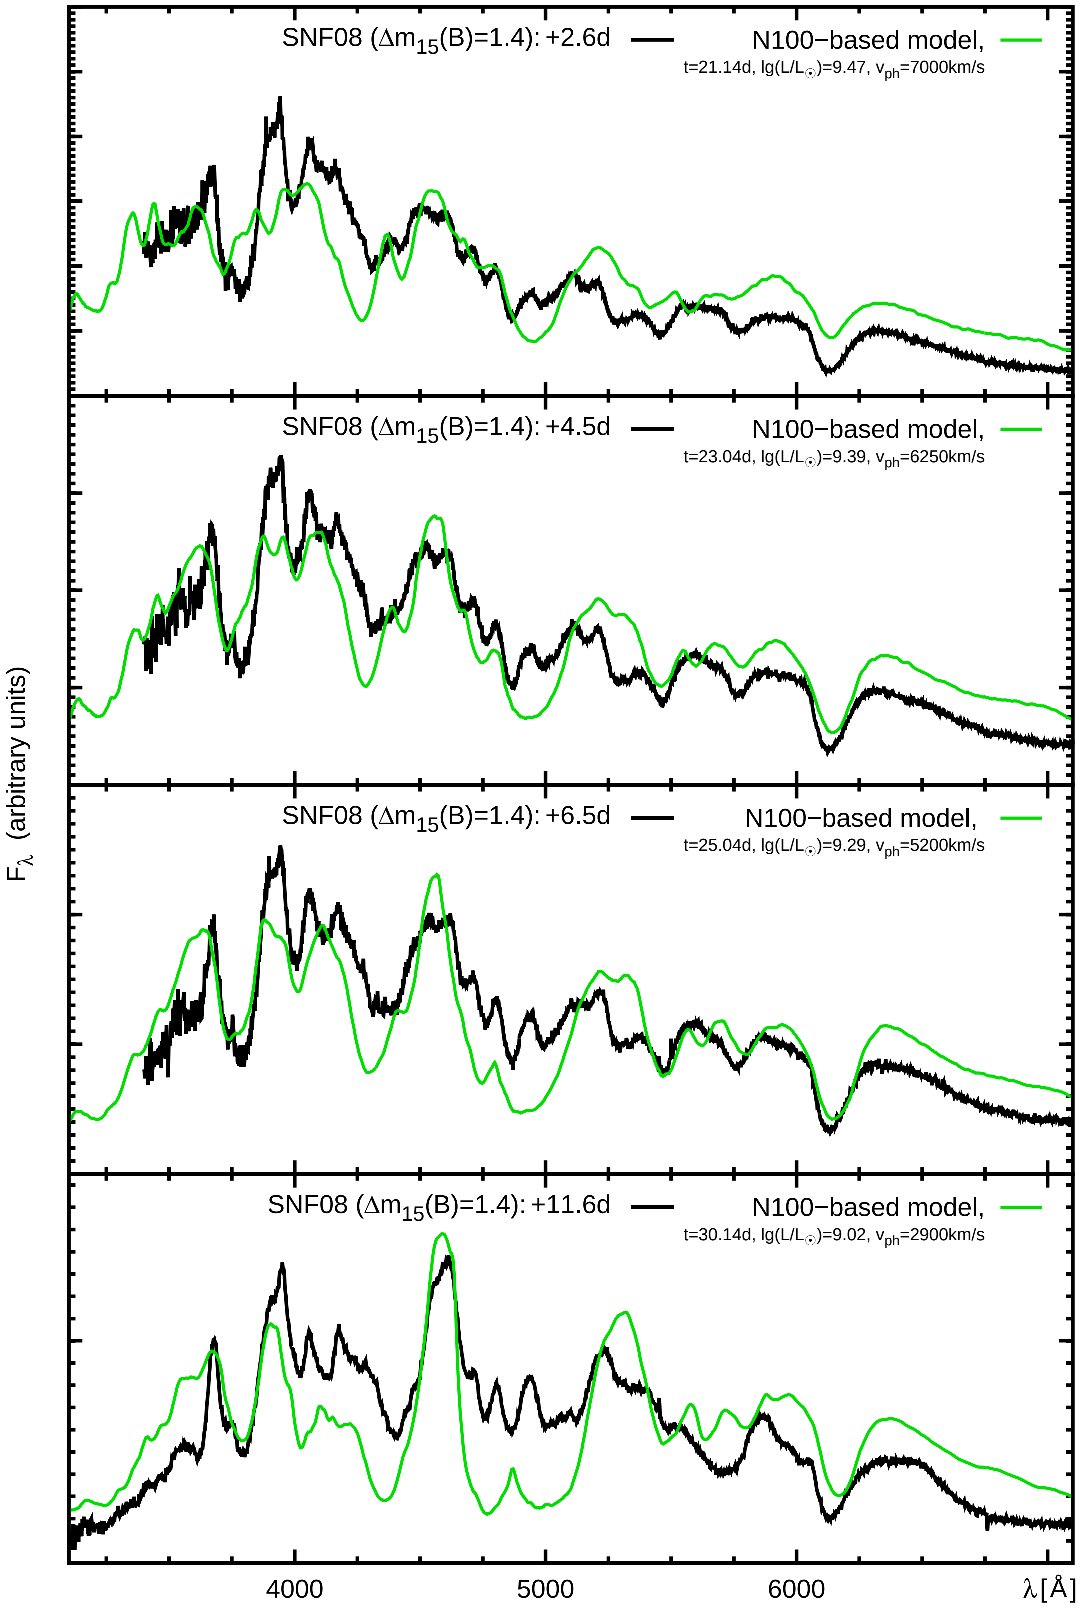


**Figure 10.** Model sequence for the 'no-Na' SN SNF 20080514-002 (green lines). The observed (low-resolution) spectra (black lines) are plotted for comparison. Analogous to Figure 1. Due to the lack of pre-maximum spectra for this SN, the fit quality is somewhat worse than for the other objects.

© 2017 The Authors. Journal compilation © 2017 RAS, MNRAS

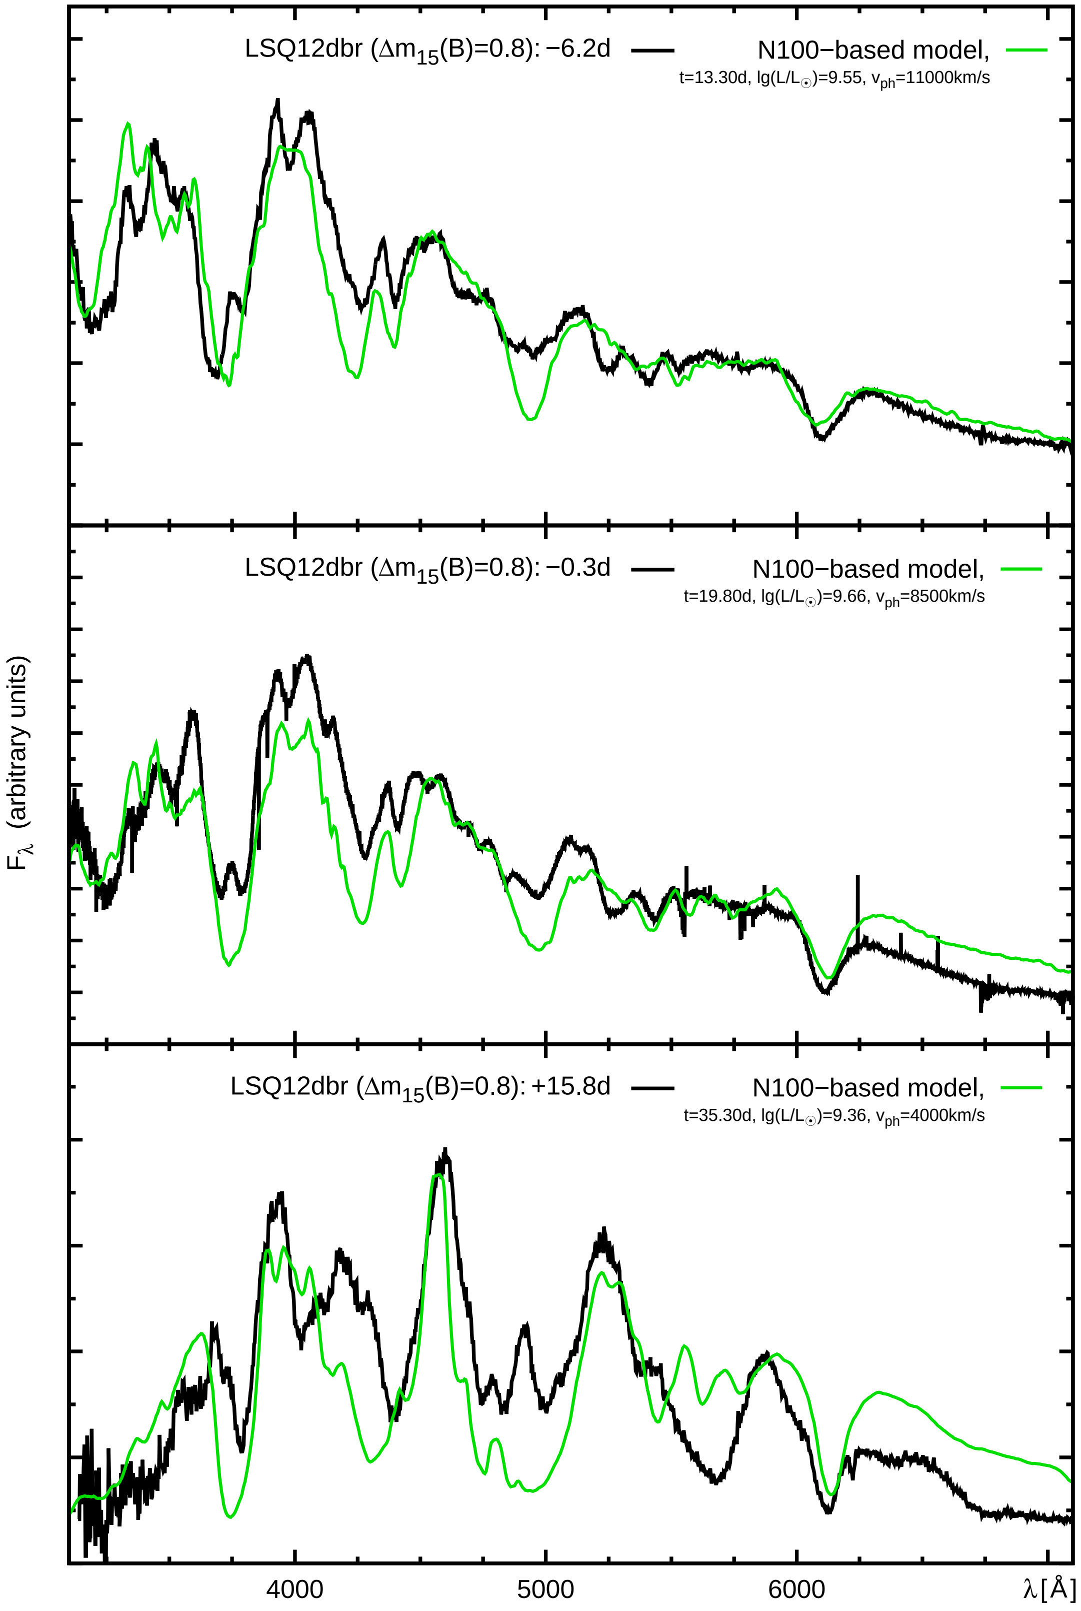


**Figure 11.** Model sequence for the 'no-Na' SN LSQ 12dbr (green lines). The observed (low-resolution) spectra (black lines) are plotted for comparison. Analogous to Figure 1.

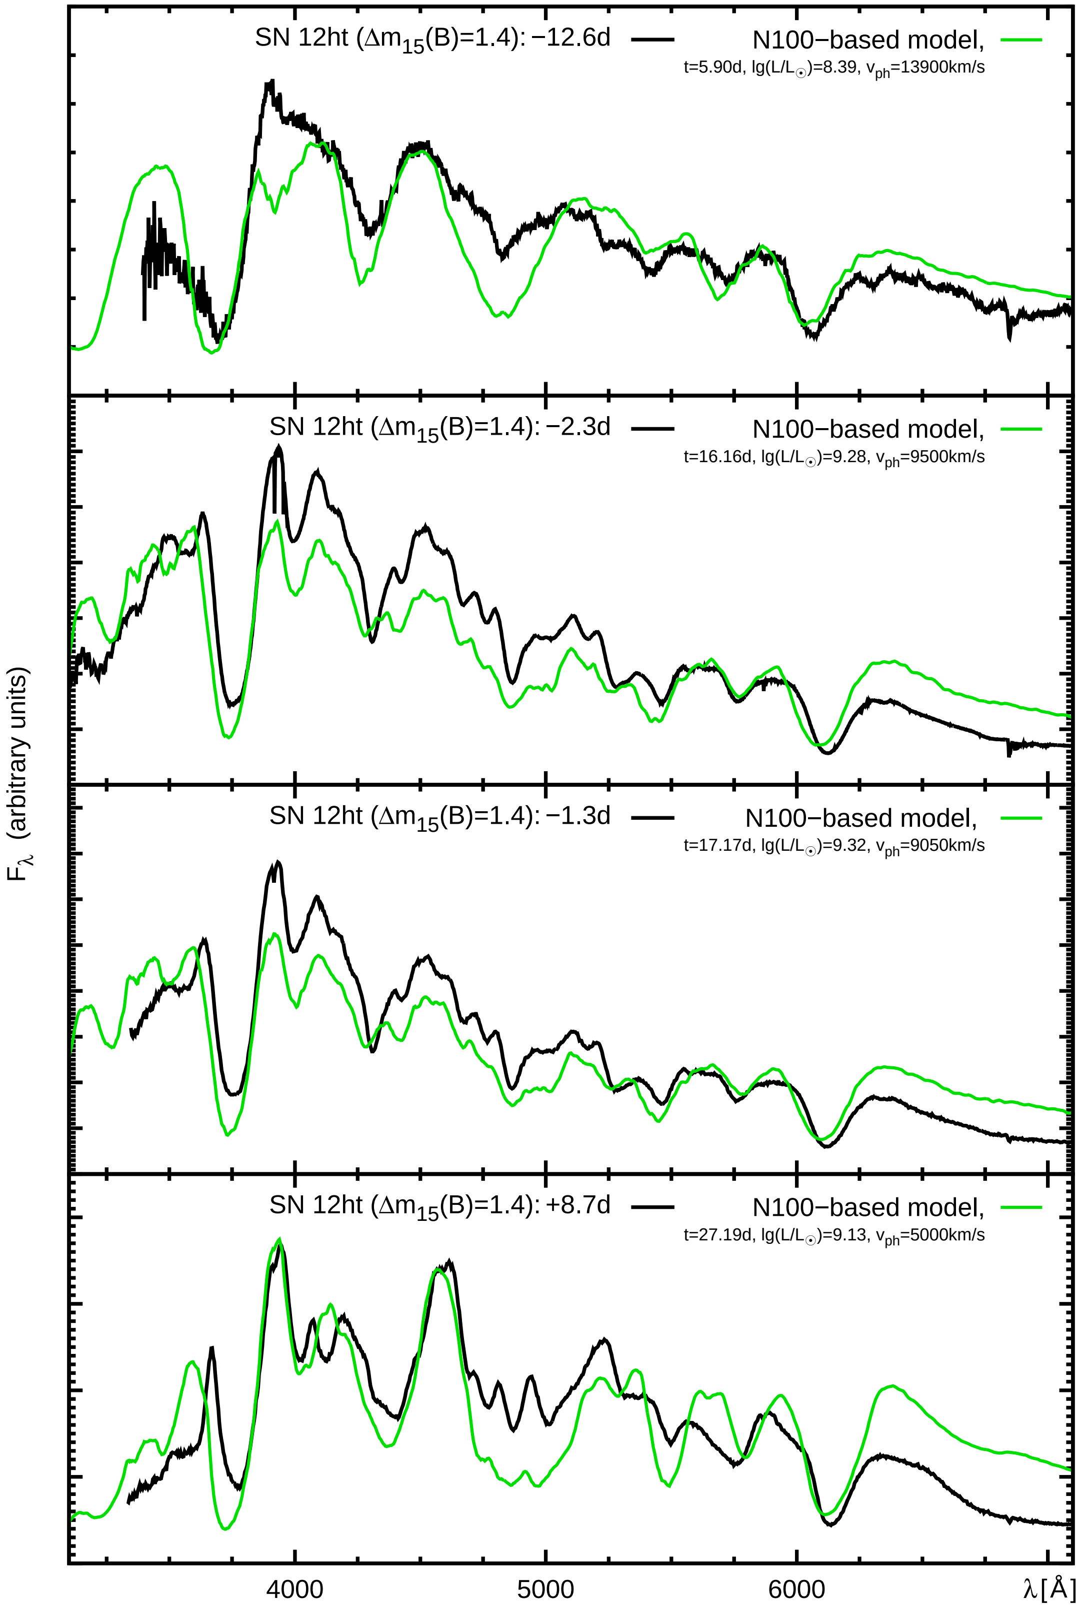


**Figure 12.** Model sequence for the 'no-Na' SN 2012ht (green lines). The observed (low-resolution) spectra (black lines) are plotted for comparison. Analogous to Figure 1.

© 2017 The Authors. Journal compilation © 2017 RAS, MNRAS

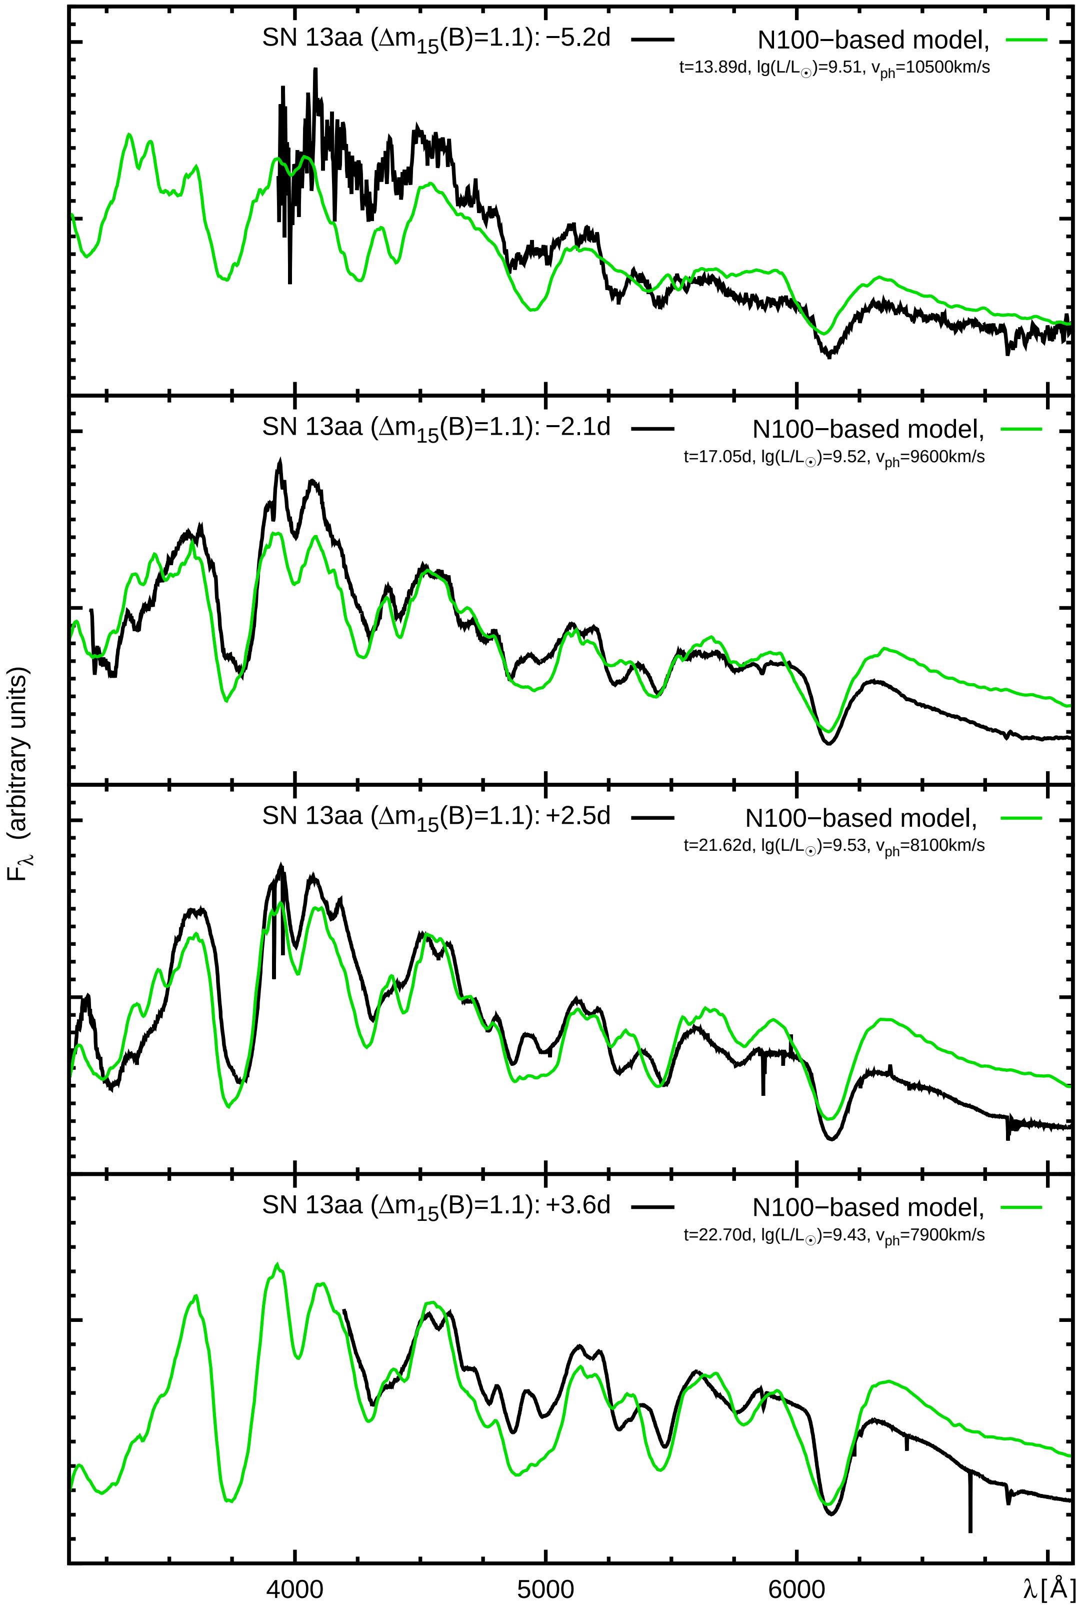


**Figure 13.** Model sequence for the 'no-Na' SN 2013aa (green lines). The observed (low-resolution) spectra (black lines) are plotted for comparison – analogous to Figure 1. For modelling SN 2013aa, we have assumed a redshift-independent distance modulus of 30.35 from LEDA (LEDA – http://leda.univ-lyon1.fr, see also acknowledgements), as with the NED redshift-dependent and redshift-independent values (larger by $\gtrsim$0.5) the ionisation equilibrium within the ejecta model was highly inconsistent with the observations.

© 2017 The Authors. Journal compilation © 2017 RAS, MNRAS

## 2 ATLAS OF ABUNDANCE DISTRIBUTIONS CORRESPONDING TO OUR SPECTRAL MODELS

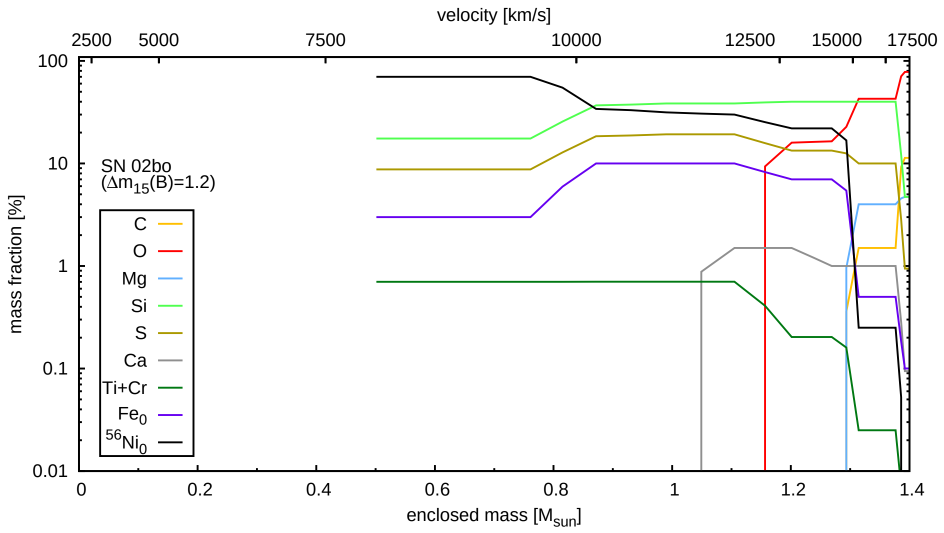


**Figure 14.** Abundance structure of our model for the 'blueshifted-Na' SN 2002bo, based on the N100 density profile. The Ni / Co / Fe abundances are given in terms of the mass fractions of $^{56}$Ni and stable Fe at $t = 0$ [$X(^{56}\mathrm{Ni}_0)$, $X(\mathrm{Fe}_0)$]. The abundances we infer for the dominant elements (O, Si, $^{56}$Ni) in SN 2002bo are similar to those inferred by Stehle et al. (2005). Remaining differences are due to our simplified modelling approach (constrained abundance mixes), and to different assumptions on the density profile and on the distance to the SN.

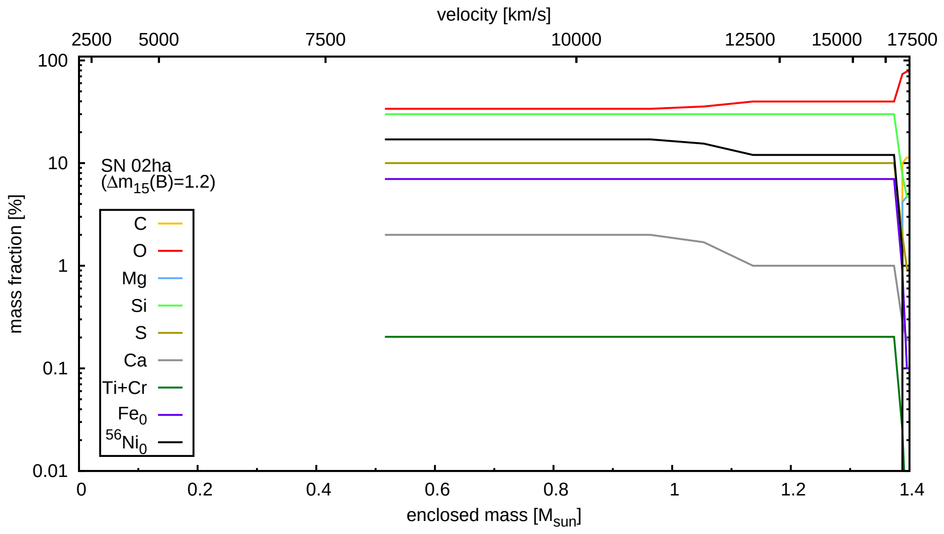


**Figure 15.** Abundance structure of our model for the 'blueshifted-Na' SN 2002ha, based on the N100 density profile. Plot analogous to Figure 14.

© 2017 The Authors. Journal compilation © 2017 RAS, MNRAS

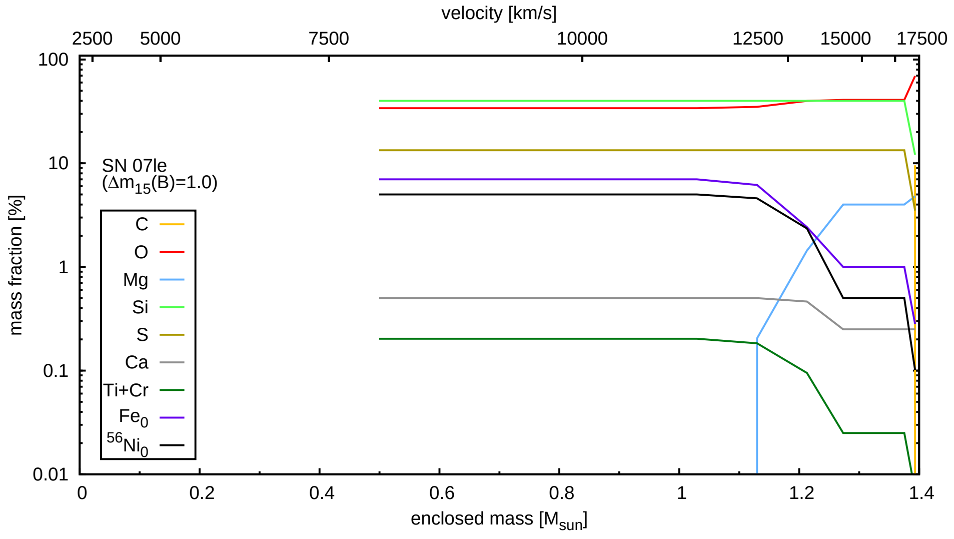


**Figure 16.** Abundance structure of our model for the 'blueshifted-Na' SN 2007le, based on the N100 density profile. Plot analogous to Figure 14.

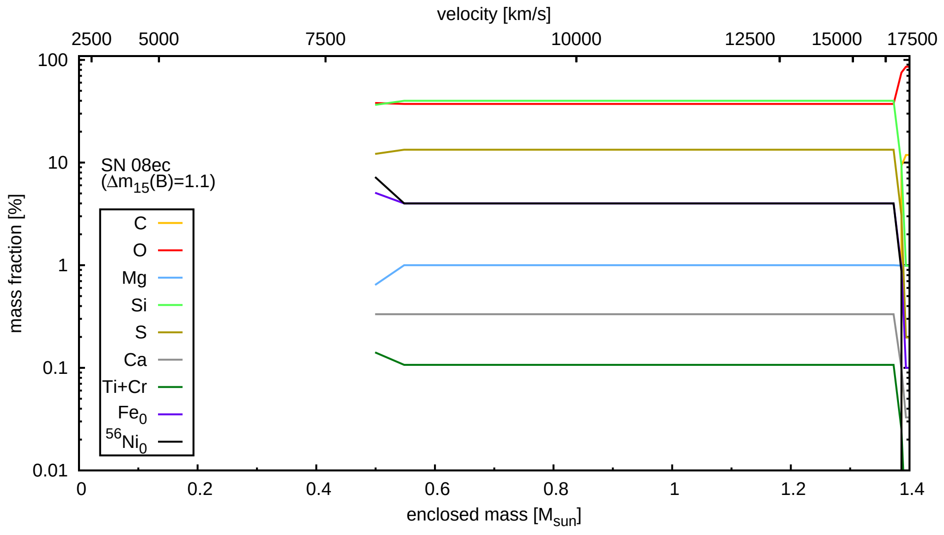


**Figure 17.** Abundance structure of our model for the 'blueshifted-Na' SN 2008ec, based on the N100 density profile. Plot analogous to Figure 14.

© 2017 The Authors. Journal compilation © 2017 RAS, MNRAS

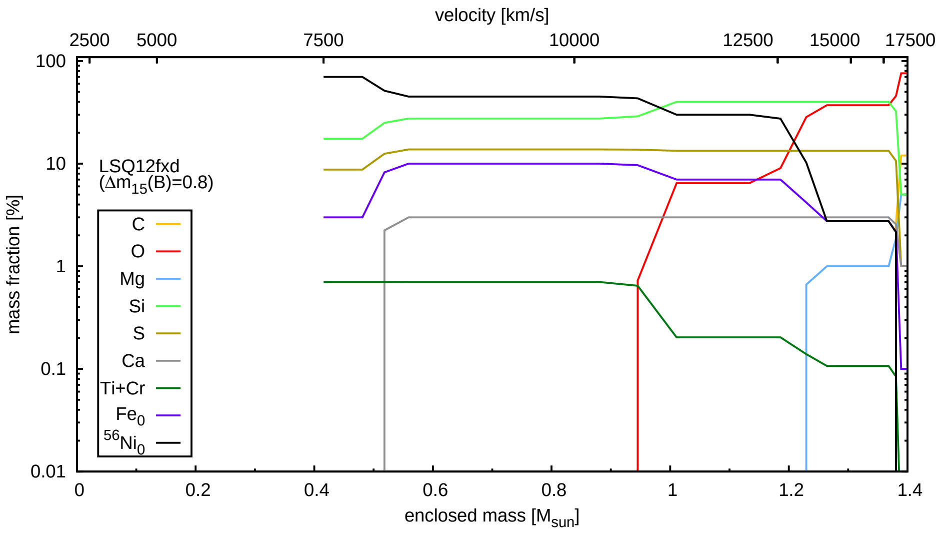


**Figure 18.** Abundance structure of our model for the 'blueshifted-Na' SN LSQ 12fxd, based on the N100 density profile. Plot analogous to Figure 14.

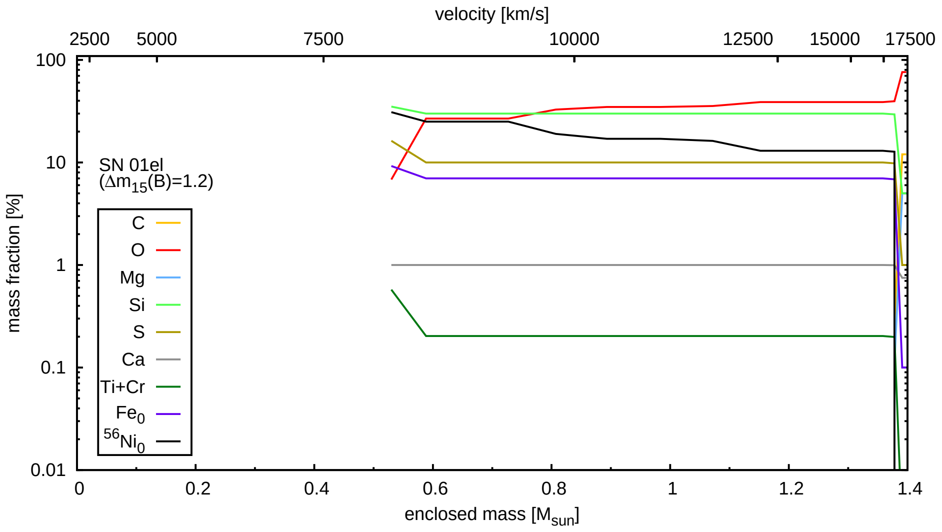


**Figure 19.** Abundance structure of our model for the 'redshifted-Na' SN 2001el, based on the N100 density profile. Plot analogous to Figure 14.

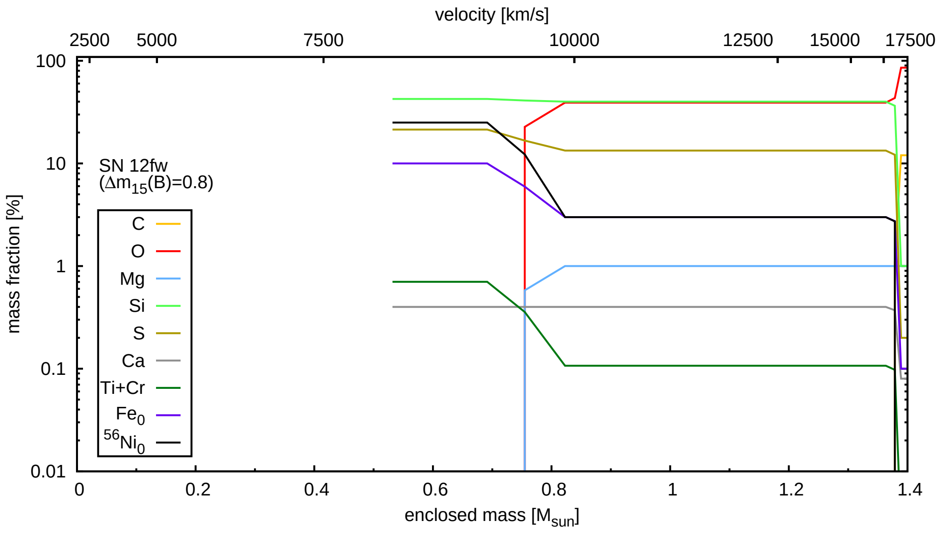


**Figure 20.** Abundance structure of our model for the 'redshifted-Na' SN 2012fw, based on the N100 density profile. Plot analogous to Figure 14.

© 2017 The Authors. Journal compilation © 2017 RAS, MNRAS

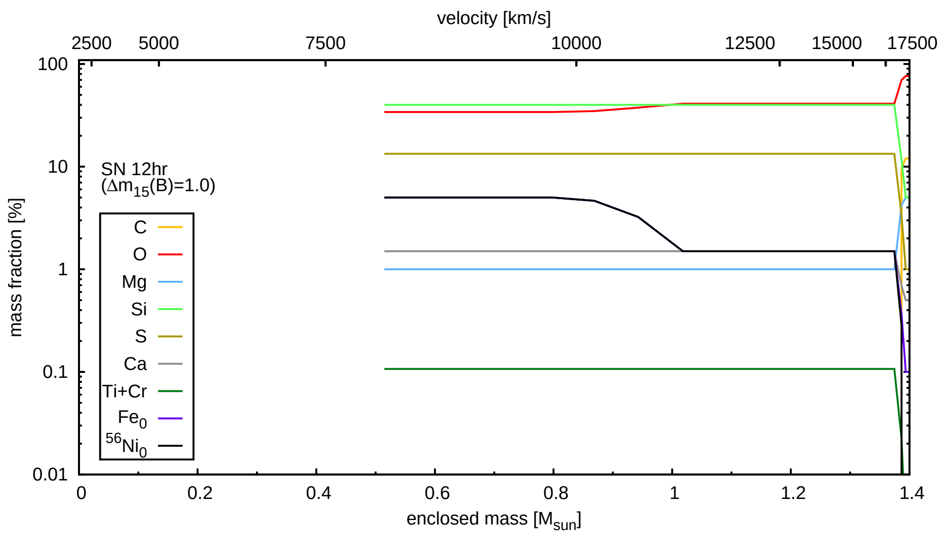


**Figure 21.** Abundance structure of our model for the 'redshifted-Na' SN 2012hr, based on the N100 density profile. Plot analogous to Figure 14.

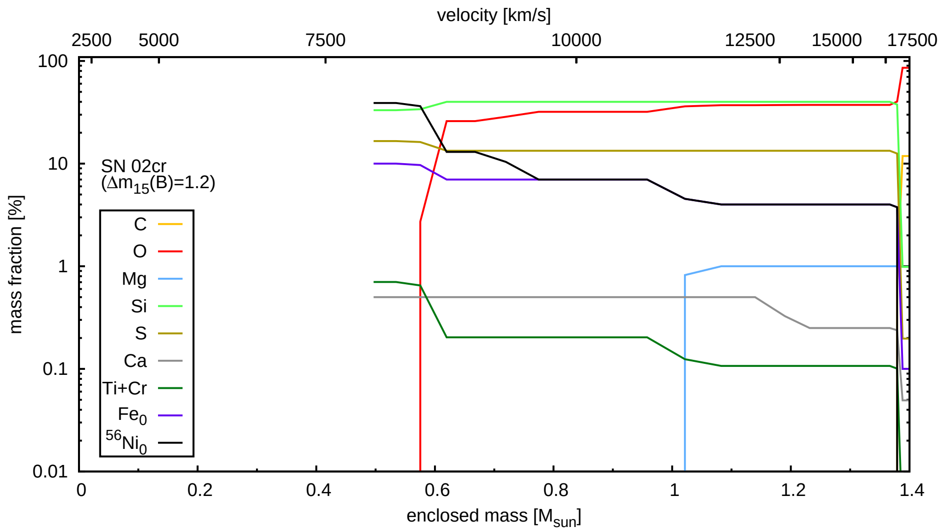


**Figure 22.** Abundance structure of our model for the 'single-Na' SN 2002cr, based on the N100 density profile. Plot analogous to Figure 14.

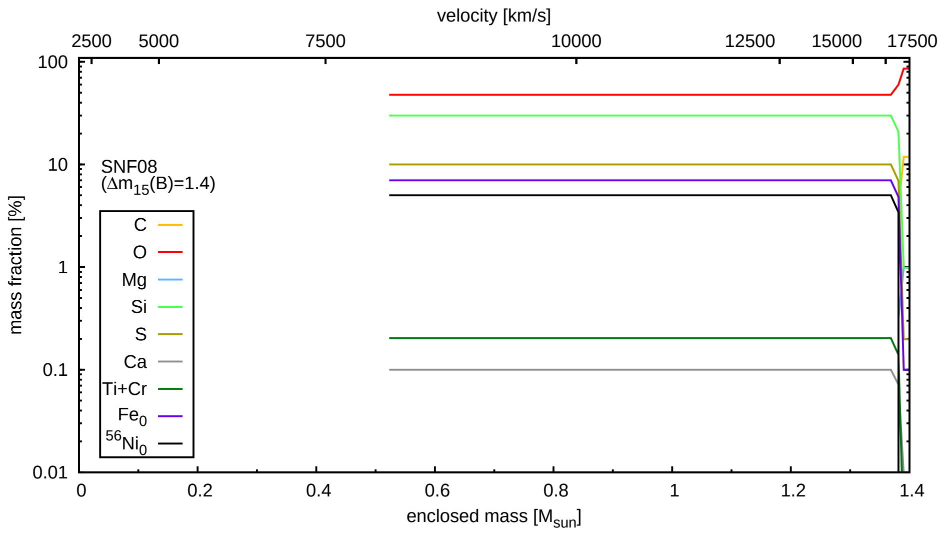


**Figure 23.** Abundance structure of our model for the 'no-Na' SN SNF 20080514-002, based on the N100 density profile. Plot analogous to Figure 14.

© 2017 The Authors. Journal compilation © 2017 RAS, MNRAS

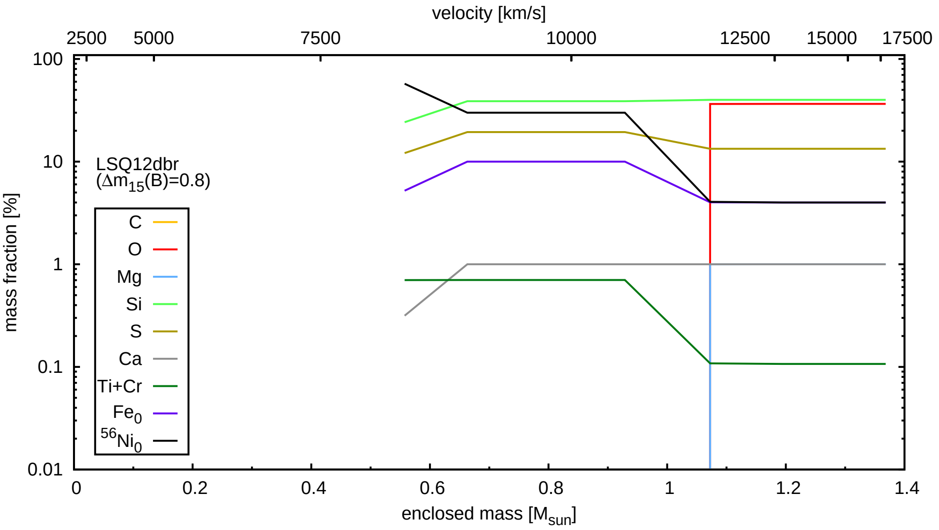


**Figure 24.** Abundance structure of our model for the 'no-Na' SN LSQ 12dbr, based on the N100 density profile. Plot analogous to Figure 14.

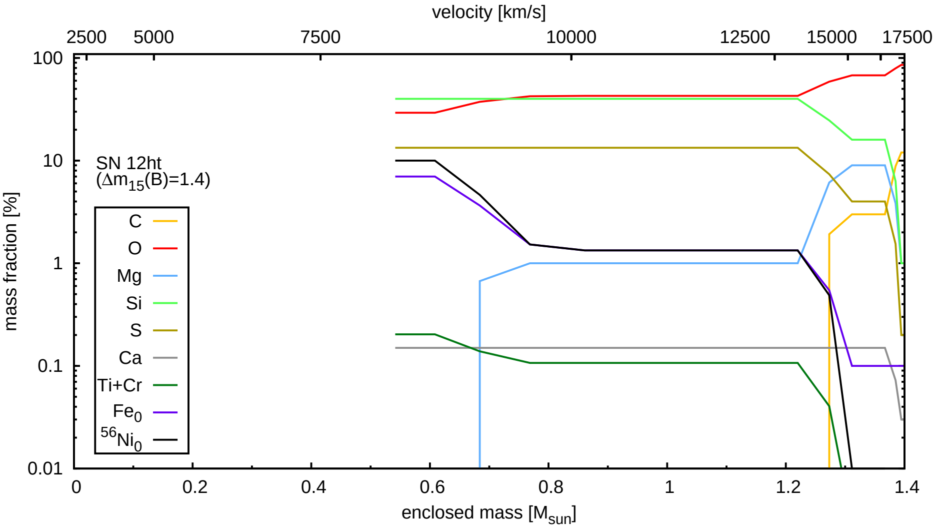


**Figure 25.** Abundance structure of our model for the 'no-Na' SN 2012ht, based on the N100 density profile. Plot analogous to Figure 14.

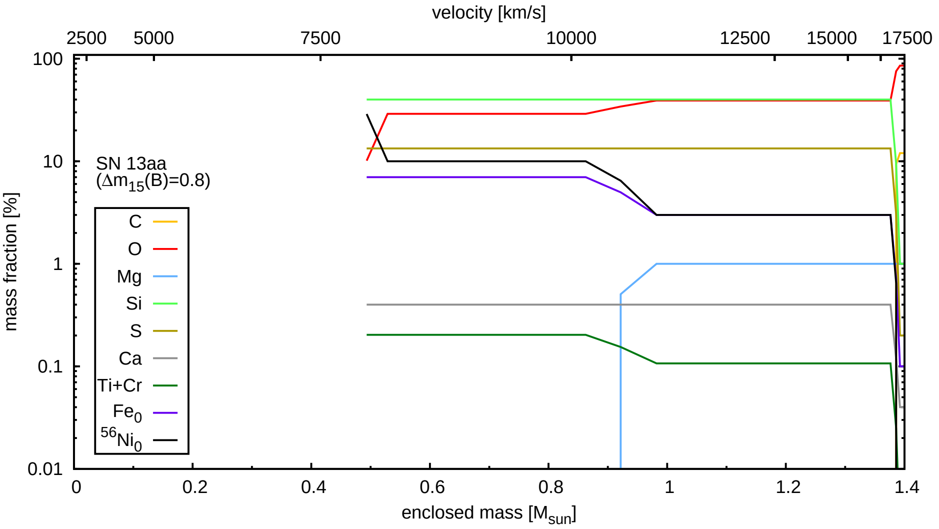


**Figure 26.** Abundance structure of our model for the 'no-Na' SN 2012ht, based on the N100 density profile. Plot analogous to Figure 14.

© 2017 The Authors. Journal compilation © 2017 RAS, MNRAS
