# Supplementary material for: Type Ia supernovae with and without blueshifted narrow Na I D lines - how different is their structure?
Source: arXiv:1707.00700 ancillary file (2017-07-03)
Supplement: Supplementary file 2 [file suppB-NaId-SN-structanalysis.pdf]

Mon. Not. R. Astron. Soc. (2017) (MN LaTeX style file v2.2)

# Supplementary material B: Type Ia supernovae with and without blueshifted narrow Na I D lines – how different is their structure?

S. Hachinger[1,2,3], F. K. Röpke[1,4], P. A. Mazzali[5,6], A. Gal-Yam[7], K. Maguire[8,9], M. Sullivan[10], S. Taubenberger[8,6], C. Ashall[5], H. Campbell[11], N. Elias-Rosa[12], U. Feindt[13], L. Greggio[12], C. Inserra[9], M. Miluzio[12,14], S. J. Smartt[9], D. Young[9]

[1]*Institut für Theoretische Physik und Astrophysik, Universität Würzburg, Emil-Fischer-Str. 31, 97074 Würzburg, Germany*
[2]*Institut für Mathematik, Universität Würzburg, Emil-Fischer-Str. 30, 97074 Würzburg, Germany*
[3]*Leibniz Supercomputing Centre (LRZ), Bavarian Academy of Sciences and Humanities, Boltzmannstr. 1, 85748 Garching b. München, Germany*
[4]*Heidelberger Institut für Theoretische Studien, Schloss-Wolfsbrunnenweg 35, 69118 Heidelberg, Germany*
[5]*Astrophysics Research Institute, Liverpool John Moores University, IC2 Liverpool Science Park, 146 Brownlow Hill, Liverpool, L3 5RF, UK*
[6]*Max-Planck-Institut für Astrophysik, Karl-Schwarzschild-Str. 1, 85741 Garching, Germany*
[7]*Benoziyo Center for Astrophysics, Weizmann Institute of Science, 76100 Rehovot, Israel*
[8]*European Organisation for Astronomical Research in the Southern Hemisphere (ESO), Karl-Schwarzschild-Str. 2, 85748 Garching b. München, Germany*
[9]*School of Mathematics and Physics, Queen's University Belfast, Belfast BT7 1NN, UK*
[10]*Physics & Astronomy, University of Southampton, Southampton, Hampshire SO17 1BJ, UK*
[11]*Institute of Astronomy, University of Cambridge, Madingley Road, Cambridge CB3 0HA, UK*
[12]*INAF - Osservatorio Astronomico di Padova, vicolo dell'Osservatorio 5, 35122 Padova, Italy*
[13]*Oskar Klein Centre, Department of Physics, Stockholm University, Albanova University Center, 10691 Stockholm, Sweden*
[14]*Instituto de Astrofisica de Canarias, C/ Vía Láctea, s/n, 38205, La Laguna, Tenerife, Spain*

**ABSTRACT**

In this supplementary appendix, we would like to calculate how likely we will actually see physical differences between our blueshifted-Na SNe Ia and other SNe Ia. More precisely, our aim is to infer the probabilities of finding 'CSM producers' and 'CSM-free systems' in our different Na subsamples, respectively (assuming that SNe Ia come from these two 'types' of progenitor systems). For simplicity, throughout this appendix we assume that the subsample statistics observed by Maguire et al. (2013) be exactly representative of reality. The results presented here have already been summarised in the main text.

## PROBABILITY OF FINDING DIFFERENCES BETWEEN Na SUBSAMPLES, ASSUMING TWO PROGENITOR CHANNELS

### 1 PHENOMENOLOGY

To start out, we recap how (and why) a sample of CSM-producing systems will look different with respect to CSM-free systems. Owing to a CSM outflow with high enough optical depth in the Na lines, blueshifted (narrow) Na I D components appear in the spectrum (as the SN is obscured by CSM-outflow material moving towards the observer – material behind or at the side of the SN is irrelevant in this context). Systems with CSM Na which have no ISM Na will thus show up as blueshifted-Na SNe (i.e. the number of blueshifted-Na objects is augmented at the expense of no-Na objects); CSM-Na systems with redshifted ISM Na will show up as SNe with red- and blueshifted Na components at the same time. Systems which have blueshifted or both blue- and redshifted ISM lines will normally remain in the respective subsample when blueshifted CSM components are added. On this basis, we will now interpret the excess of blueshifted-Na SNe found in the literature.

### 2 OBSERVED STATISTICS

In their fine classification (their Table 4), Maguire et al. (2013) find *ten '(only-)blueshifted-Na' SNe, four '(only-)redshifted-Na' SNe, seven 'blue-and-redshifted-Na' SNe, and ten 'no-Na' SNe* within their full (combined) sample. They classify one object as 'symmetric-Na', which we exclude here for simplicity; thus we consider a *total of 31 objects.* The excess of blueshifted-Na SNe with respect to redshifted-Na ones (a difference of six objects) has two reasons: most obviously, 'additional' blueshifted CSM Na components appearing in CSM producers make objects with no ISM Na line show blueshifted Na. Secondly, CSM components make objects with redshifted ISM Na appear as blue-and-redshifted-Na SNe (meaning that less redshifted-Na SNe are observed).

© 2017 The Authors. Journal compilation © 2017 RAS

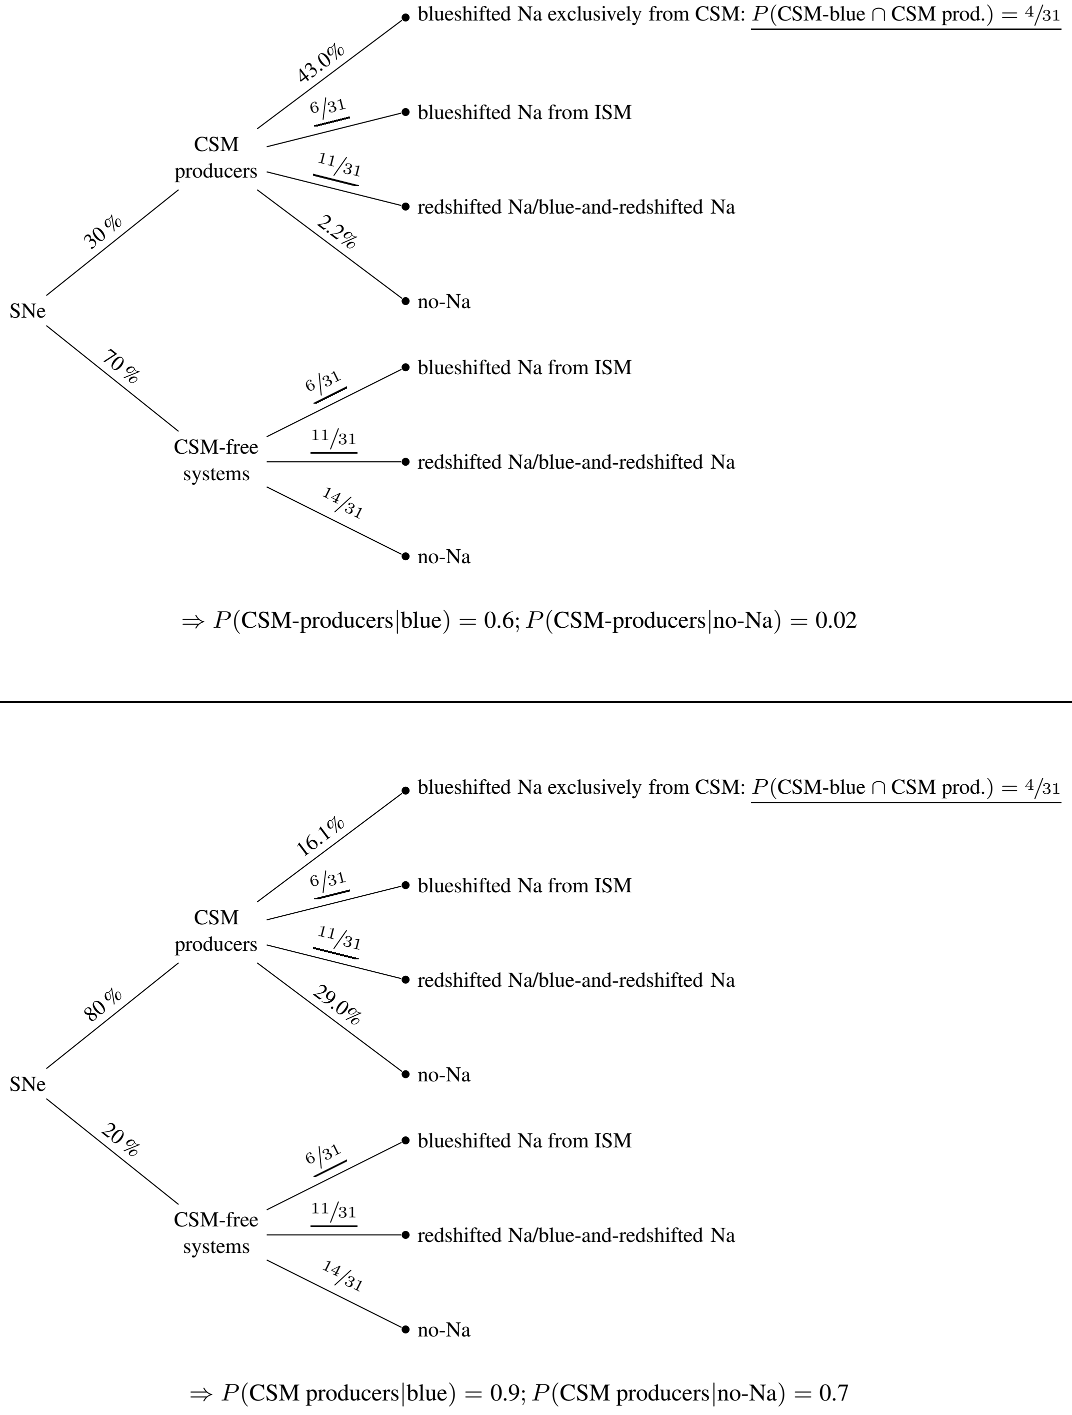


**Figure 1.** Example probability trees and resulting conditional probabilities for finding CSM producer SNe Ia among different Na subsamples. For the *upper tree*, we assume 30% of SN Ia progenitors to be 'CSM producers'; 80% in the *lower tree*. The underlined 'approximate probabilities' (relative frequencies) are from the 'combined sample' of Maguire et al. (2013) (cf. end of Section 2). Note that the probabilities of $6/31$ and $11/31$ for blueshifted-ISM-Na and redshifted-/blue-and-redshifted-ISM-Na objects, respectively, can be used for CSM-producers as well as other systems as we assume that ISM-Na lines appear in all systems with the same likelihood (cf. text). With the underlined numbers fixed, the rest of the numbers is computed using the formula $P(B|A) = P(A \cap B)/P(A)$ and demanding that probabilities behind each node add up to 1.

We now assume that the numbers of SNe 'converted' (by the appearance of CSM lines) in these two ways, respectively, scale proportionally with the quantity of no-Na vs. redshifted-Na SNe (10 vs. 4 –of 14 in total – i.e. a normalised ratio of 0.7:0.3)[1]. Then, we can calculate that from the difference of 6 SNe between the blueshifted-Na and redshifted-Na subsample size (as mentioned at the beginning of the section), $6 \times 0.7 \sim 4$ SNe are statistically due to added blueshifted components. This means that $6 \times 0.3 \sim 2$ redshifted-Na SNe are missing as they now appear as blue-and-redshifted-Na SNe.

If 4 SNe out of Maguire's sample show blueshifted lines caused by CSM only ('converted objects', as calculated), and 10 show no lines at all (Maguire's 'no-Na' SNe), 17 SNe of the full sample remain which show lines made by ISM (additional CSM lines may be present). Of these 17 SNe, 7 SNe show mixed 'blue-and-redshifted' lines, 6 SNe show blueshifted Na lines only, and 4 SNe show redshifted Na lines only.

To summarise, we arrive at the following probabilities of showing Na I D lines, if we take the relative frequencies among the 31 objects considered as representative:

- $^4/_{31}$ of *all* SNe show blueshifted Na I D lines from the CSM and at the same time have no ISM lines, i.e. they originate only from CSM-producing systems;
- $^{10}/_{31}$ of *all* SNe show no Na I D line;
- $^6/_{31}$ of *all* SNe show blueshifted Na I D lines (and no redshifted ones) from the ISM[2] (as an approximation good enough for our purposes, this may be considered to hold independently for each progenitor type, i.e. $^6/_{31}$ of the *CSM producers*, and of the *CSM-free systems*, respectively);
- $^{11}/_{31}$ of all SNe (or, again, in good approximation of *CSM producer-SNe* as well as *CSM-free SNe*), show redshifted Na I D lines from the ISM (with possible additional blueshifted CSM-/ISM-components). Out of these, 2 objects ($^2/_{31}$ of all SNe) have only redshifted ISM Na I D, but an additional blueshifted CSM component, making them appear as blue-and-redshifted-Na SNe.

## 3 THE FRACTION OF CSM-PRODUCERS IN NO-NA VS. BLUESHIFTED-NA SYSTEMS

With the information gathered, we can readily compute the probability of finding CSM-producer systems among blueshifted-Na SNe and among no-Na SNe (probabilities for the redshifted-Na and red-and-blueshifted-Na subsample will be derived in Section 4). The probabilities we calculate will critically depend on the *initial fraction of SNe coming from CSM-producer systems*. As this fraction is unknown, we treat and interpret two arbitrarily-chosen example cases here, in which a minority (30%) or a majority (80%) of SNe-Ia come from CSM-producing systems.

For making the computations more intuitive, we first construct probability trees. Figure 1 shows two versions of the same tree, assuming 30% or 80% of all SNe Ia to generally emerge from CSM-producer systems (the rest comes from CSM-free systems).

CSM-producer SNe are split up according to their narrow Na I D properties into no-Na, redshifted-/blue-and-redshifted-Na, 'blueshifted Na from ISM', and 'blueshifted Na exclusively from CSM' subgroups; for CSM-free SNe the blueshifted-CSM-Na subgroup does not exist. Note that 'blueshifted Na from ISM' SNe may sometimes have have additional CSM components, which are irrelevant in our context. The only relevant distinguishing criterion here is that 'blueshifted Na exclusively from CSM' SNe appear 'blueshifted Na' *because of the CSM lines*, and thus are part of the excess of blueshifted-Na objects (over redshifted-Na ones) created by CSM-producing progenitors.

In Figure 1, the numbers from the end of Section 2 have been typeset underlined; the rest of the numbers appearing in the probability trees is calculated from the formula $P(B|A) = P(A \cap B)/P(A)$ and from the sum rule (probabilities behind each node have to add up to one).

The probabilities of finding CSM-producer objects in different subsamples are then calculated using Bayes' theorem for the conditional probability $P(A|B)$ of an event $A$ under the assumption that an event $B$ has occurred:

$$P(A|B) = \frac{P(B|A)\,P(A)}{P(B)} = \frac{P(B|A)\,P(A)}{P(B|A)P(A) + P(B|\bar{A})P(\bar{A})}.$$

Here, $\bar{A}$ is the complement of the event $A$ and the conditional probabilities are per convention such that $P(A|B) + P(\bar{A}|B) = 1$. As an example, we calculate the conditional probability of finding a CSM-producer in the subsample with blueshifted Na I D (from CSM and/or ISM) as:

$$\begin{aligned} &P(\text{CSM-producers}|\text{blue}) = \\ &P(\text{blue}|\text{CSM-producers}) \times P(\text{CSM-producers})/ \\ &[P(\text{blue}|\text{CSM-producers}) \times P(\text{CSM-producers}) + \\ &P(\text{blue}|\text{CSM-free systems}) \times P(\text{CSM-free systems})]\,, \end{aligned}$$

which numerically – for the case that 30% of all SNe are CSM producers (Figure 1, upper panel) – gives:

$$\begin{aligned} &P(\text{CSM-producers}|\text{blue}) \approx \\ &(43.0\% + {}^6/_{31}) \times 30\%/ \\ &[(43.0\% + {}^6/_{31}) \times 30\% + {}^6/_{31} \times 70\%)] \approx 0.6. \end{aligned}$$

Note that the event 'blue' has contributions from two sub-branches of the CSM-producer branch in the probability tree (the blueshifted-CSM-Na sub-branch with a conditional probability of 43.0%, and the blueshifted-ISM-Na sub-branch with its conditional probability of $^6/_{31}$); from the CSM-free branch only one sub-branch (conditional probability $^6/_{31}$) contributes. The conditional probability $P(\text{CSM-producers}|\text{no-Na})$ is calculated analogously. The respective results are given in Figure 1.

It turns out that the CSM-producer fraction in different Na I D subsamples depends strongly on the general production fraction of SNe Ia from the different channels. The lower the rate of CSM producers, the larger the difference between the subsamples. If less than 30% of all SNe were from CSM producers, these systems would practically *always* have to produce a CSM line (i.e. they would not make no-Na SNe) in order to explain the excess

[1] Here, the assumption of a 'proportional' decrease (in the no-Na and redshifted-Na subsample by 'added' CSM lines) means that the ratio of redshifted-Na to no-Na SNe is the same whether we look at the subsample sizes before or after the decrease. It is essentially equivalent with the assumption that objects which would be in the redshifted-Na and no-Na groups with just their ISM Na lines are equally probable to show added CSM lines (thus being counted as red-and-blueshifted-Na and blueshifted-Na objects by the observer).

[2] For us, it is irrelevant whether these SNe show additional lines due to the CSM; it is only relevant that these objects are *not* part of the excess blueshifted-Na objects created by CSM-producing progenitor systems (cf. Section 3) .

© 2017 The Authors. Journal compilation © 2017 RAS, MNRAS

of (only-)blueshifted-Na objects with respect to (only-)redshifted ones [i.e. the four blueshifted-CSM-Na objects).

Our statistical model has a further noteworthy aspect: It puts a strict lower limit to the CSM-producer fraction, below which the model is unable to explain the observations (i.e. the excess of blueshifted-Na objects). This lower limit is $\sim 28.6\%$.

## 4 THE FRACTION OF CSM PRODUCERS IN REDSHIFTED-(ONLY-)NA SNE

When calculating the fraction of CSM-producers among redshifted-(only-)Na SNe, we have to consider the fact that CSM-producing systems will produce less redshifted-Na SNe, and more blue-and-redshifted-Na SNe instead. We consider this situation in a more detailed probability tree (this time only for the 80%/20% CSM-producer/CSM-free case: Figure 2); all calculations follow the principles mentioned above and use the numbers mentioned in Section 2.

It turns out that the probability of finding CSM-producers among only-redshifted-Na SNe is equal to that of finding them among no-Na SNe (within rounding errors) – i.e. 0.7 for the 80%/20% case, and a few per cent for the 30%/70% case, respectively. This is the consequence of our earlier assumption that the only-redshifted-Na subsample and the no-Na subsample are reduced 'at equal rates' (i.e. proportionally to their magnitude) among the CSM-producer systems.

## References

Maguire K., et al., 2013, MNRAS, 436, 222

© 2017 The Authors. Journal compilation © 2017 RAS, MNRAS

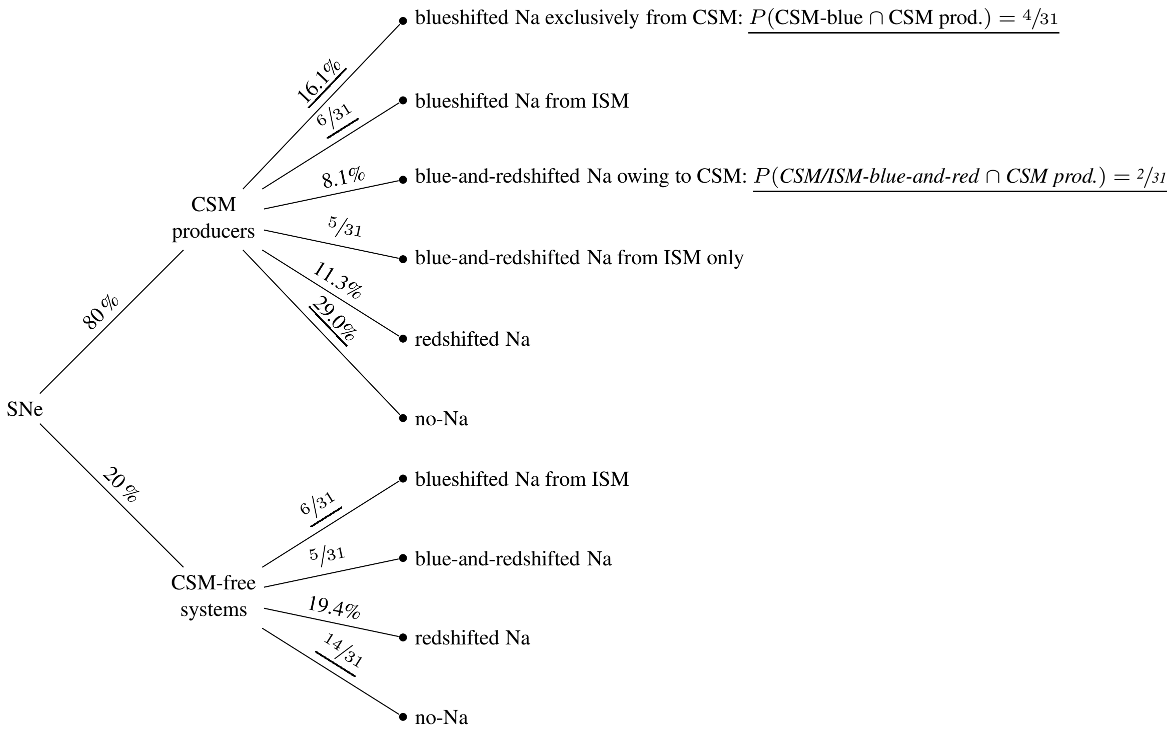


$$\Rightarrow P(\text{CSM producers}|\text{blue}) = 0.9;\ P(\text{CSM producers}|\text{red}) = 0.7$$

**Figure 2.** Extended probability tree (cf. lower tree in Figure1) and conditional probability for finding CSM producer SNe Ia among (only-)redshifted-Na SNe. We assume 80% of the progenitor systems to be CSM producers. The tree reflects the fact that CSM-producing systems make more blue-and-redshifted-Na SNe at the expense of redshifted-Na ones. The underlined numbers are the same as in Figure 1; the *italic-underlined* probability is additionally extracted from the end of Section 2. From the given numbers, one calculates branch probabilities of 8.1% for the blue-and-redshifted-CSM/ISM-Na case, and $5/31$ for the blue-and-redshifted-ISM-Na cases (in order to arrive at seven blue-and-redshifted-Na SNe in total). The branch probabilities of 11.3% and 19.4% for only-redshifted-Na SNe then derive from the constraint that probabilities behind each node add up to 1.

© 2017 The Authors. Journal compilation © 2017 RAS, MNRAS
